# Supplementary material for: Noise-Resilient Quantum Metrology
Source: arXiv:2509.25384 ancillary file (2026-05-05)
Supplement: Supplementary file 1 [file supplementary_information.pdf]

# Supplementary information for: Continuous-Wave Interferometry at the Heisenberg Limit

Hudson A. Loughlin,<sup>1,\*</sup> Melissa A. Guidry,<sup>1</sup> Jacques Ding,<sup>1,2</sup> Masaya Ono,<sup>1,3</sup> Malo Le Gall,<sup>1</sup>  
Benjamin Lou,<sup>1</sup> Eric Oelker,<sup>1</sup> Xinghui Yin,<sup>1</sup> Vivishek Sudhir,<sup>1,4</sup> and Nergis Mavalvala<sup>1</sup>

<sup>1</sup>*LIGO Laboratory, Massachusetts Institute of Technology, Cambridge, MA 02139, USA*

<sup>2</sup>*Laboratoire Astroparticule et Cosmologie, Université Paris Cité, Paris, 75000, France*

<sup>3</sup>*Department of Physics, The University of Tokyo, Bunkyo, Tokyo, 113-0033, Japan*

<sup>4</sup>*Department of Mechanical Engineering, Massachusetts Institute of Technology, Cambridge, MA 02139, USA*

(Dated: September 29, 2025)

## CONTENTS

|                                                                                 |    |
|---------------------------------------------------------------------------------|----|
| I. Notations, conventions                                                       | 2  |
| A. Fields and operators in quantum and classical optics                         | 2  |
| B. Properties of the Fourier transform                                          | 3  |
| C. Matrix formalism                                                             | 3  |
| 1. Propagation in Free space                                                    | 3  |
| 2. Beam splitter                                                                | 3  |
| D. Spectral densities                                                           | 3  |
| E. Some properties of $\text{rect}(x)$                                          | 4  |
| II. Theory: Spectral Quantum Cramer Rao bound for a Mach-Zehnder interferometer | 5  |
| A. Propagation of squeezed states through a Mach-Zehnder interferometer         | 5  |
| B. Spectral Quantum Cramer-Rao bound for two-mode squeezed field input          | 6  |
| C. Spectral Quantum Cramer-Rao bound for a coherent and squeezed vacuum input   | 8  |
| III. Optimal estimator                                                          | 10 |
| A. Proof that the estimator is unbiased                                         | 11 |
| B. Proof of saturability of spectral QCRB                                       | 11 |
| C. Proof that the optimal estimator corresponds to the MLE                      | 12 |
| IV. Control of the squeezed fields using Coherent Locking Fields                | 13 |
| A. Notations                                                                    | 13 |
| B. The CLF-Pump loops                                                           | 15 |
| C. The Squeezing Angle Control loop                                             | 15 |
| D. MZI differential arm length lock                                             | 16 |
| E. CLF-LO loop for Homodyne Detectors                                           | 16 |
| V. Experimental Calibration Measurements                                        | 17 |
| A. Homodyne Detectors and Squeezing Measurements                                | 17 |
| B. Classical Calibration of Phase Modulation Tone                               | 18 |
| C. Estimator Linearity                                                          | 18 |
| VI. Symmetry and Stability Criteria for Accepting Data Points                   | 19 |
| References                                                                      | 21 |

---

\* [HUDSON1@MIT.EDU](mailto:HUDSON1@MIT.EDU)

## I. NOTATIONS, CONVENTIONS

### A. Fields and operators in quantum and classical optics

The quantized electric field operator with carrier frequency  $\omega_\ell$ , at location  $(x, y, z)$ , and time  $t$ , is given by [1, 2]

$$\hat{\mathbf{E}}(t) = \mathbf{u}(x, y, z) E_0(\omega_\ell) \left( \hat{a}(t) e^{-i\omega_\ell t} + \hat{a}^\dagger(t) e^{i\omega_\ell t} \right), \quad (1)$$

where  $\mathbf{u}(x, y, z)$  is a dimensionless factor encoding the field's spatial mode shape and polarization, and  $E_0(\omega_\ell) = \sqrt{2\pi\hbar\omega_\ell/(\mathcal{A}c)}$  is a normalization constant such  $\hat{a}(t)$  has the dimension of the square root of photon number flux.

We denote the magnitude electric field operator, normalized to its mode profile, at a fixed point in space by  $\hat{E}(t)$ , which is then given by

$$\hat{E}(t) = E_0(\omega_\ell) \left( \hat{a}(t) e^{-i\omega_\ell t} + \hat{a}^\dagger(t) e^{i\omega_\ell t} \right). \quad (2)$$

Defining the amplitude,  $\hat{q}(t)$ , and phase,  $\hat{p}(t)$ , field quadratures by

$$\hat{q}(t) = \frac{\hat{a}(t) + \hat{a}^\dagger(t)}{\sqrt{2}}, \quad \hat{p}(t) = i \frac{\hat{a}^\dagger(t) - \hat{a}(t)}{\sqrt{2}}, \quad (3)$$

we can write eq. (2) in quadrature form as

$$\hat{E}(t) = \sqrt{2} E_0(\omega_\ell) [\hat{q}(t) \cos(\omega_\ell t) + \hat{p}(t) \sin(\omega_\ell t)]. \quad (4)$$

From now on, we will use the shorthand notation  $E_0 := E_0(\omega_\ell)$ . Beware of the factor  $\sqrt{2}$  on the amplitude, which comes from the convention for the quadratures.

Many of the effects we will study are more naturally understood in the frequency domain than in the time domain. We define the Fourier transform of a (not necessarily Hermitian) operator  $\hat{A}(t)$  by

$$\hat{A}[\Omega] = \int_{-\infty}^{+\infty} \hat{A}(t) e^{i\Omega t} dt. \quad (5)$$

Its inverse is given by

$$\hat{A}(t) = \int_{-\infty}^{+\infty} \hat{A}[\Omega] e^{-i\Omega t} \frac{d\Omega}{2\pi} \quad (6)$$

The total field can then be written as

$$\hat{E}(t) = E_0 \left( e^{-i\omega_\ell t} \int_{-\infty}^{+\infty} \hat{a}[\Omega] e^{-i\Omega t} \frac{d\Omega}{2\pi} + e^{i\omega_\ell t} \int_{-\infty}^{+\infty} \hat{a}[\Omega]^\dagger e^{i\Omega t} \frac{d\Omega}{2\pi} \right) \quad (7)$$

To model a classical field, we assume that  $\hat{a}[\Omega]$  is composed of a mean value  $2\pi\bar{a} \in \mathbb{C}$  at some frequency  $\Omega_0$  from the carrier, and a fluctuating part  $\delta\hat{a}[\Omega]$ :

$$\hat{a}[\Omega] = 2\pi\delta[\Omega - \Omega_0] |\bar{a}| e^{i\phi_0} + \delta\hat{a}[\Omega] \quad (8)$$

where  $\phi_0 = \arg \bar{a}$  is the phase of the mean field. Indeed, under such prescription, since  $\langle \delta\hat{a}[\Omega] \rangle = 0$  (we work in the Heisenberg frame and the averages are taken with respect to the vacuum state at all frequencies), the classical field  $E(t)$  is the mean value of the quantum field  $\hat{E}(t)$  of eq. (7):

$$E(t) = \langle \hat{E}(t) \rangle = E_0 |\bar{a}| \left( e^{-i[(\omega_\ell + \Omega_0)t + \phi_0]} + e^{i[(\omega_\ell + \Omega_0)t + \phi_0]} \right) = 2E_0 |\bar{a}| \cos[(\omega_\ell + \Omega_0)t + \phi_0] \quad (9)$$

Or in quadrature form with respect to the carrier,

$$E(t) = \sqrt{2} E_0 [q(t) \cos(\omega_\ell t) + p(t) \sin(\omega_\ell t)] \quad (10)$$

with

$$q(t) = \sqrt{2} |\bar{a}| \cos(\Omega_0 t + \phi_0) \quad (11)$$

$$p(t) = -\sqrt{2} |\bar{a}| \sin(\Omega_0 t + \phi_0). \quad (12)$$

## B. Properties of the Fourier transform

We note that the Fourier transform of the conjugate is distinct from the conjugate of the Fourier transform. The two are related by

$$A^*[\Omega] = A[-\Omega]^*. \quad (13)$$

With our Fourier transform conventions, the convolution is related to the product of its Fourier transform by

$$\int_{-\infty}^{\infty} dt e^{i\Omega t} A(t)B(t) = \int_{-\infty}^{\infty} \frac{d\Omega'}{2\pi} A[\Omega']B[\Omega - \Omega'], \quad (14)$$

$$\int_{-\infty}^{\infty} \frac{d\Omega}{2\pi} e^{-i\Omega t} A[\Omega]B[\Omega] = \int_{-\infty}^{\infty} dt' A(t')B(t - t'). \quad (15)$$

## C. Matrix formalism

### 1. Propagation in Free space

We represent a propagation over a length  $L$  by a matrix map on the quadratures such that  $\mathbf{x}^{\text{out}}[\Omega] = e^{i\Omega\tau} \mathbf{R}(\phi) \mathbf{x}^{\text{in}}[\Omega]$  with  $\tau = L/c$  and  $\phi = \omega_0\tau$ . The rotation matrix is conventionally defined as  $\mathbf{R}(\phi) = \begin{bmatrix} \cos \phi & -\sin \phi \\ \sin \phi & \cos \phi \end{bmatrix}$ .

In our experiment, we always have  $L \lesssim 1$  m and the frequencies of the signal satisfy  $\Omega \lesssim 1$  MHz, so  $\Omega\tau \ll 1$ , which we neglect in the rest of the paper. Thus the propagation is simply  $\mathbf{x}^{\text{out}} = \mathbf{R}(\phi) \mathbf{x}^{\text{in}}$ .

If two modes accumulate some different phases  $\phi_1$  and  $\phi_2$ , their propagation matrix reads, in the in the basis  $\hat{\mathbf{x}} = [q_1, p_1, q_2, p_2]^T$ :

$$\hat{\mathbf{x}}^{\text{out}} = \mathbf{R}(\phi_1, \phi_2) \hat{\mathbf{x}}^{\text{in}} := \begin{bmatrix} \mathbf{R}(\phi_1) & \mathbf{0} \\ \mathbf{0} & \mathbf{R}(\phi_2) \end{bmatrix} \hat{\mathbf{x}}^{\text{in}} \quad (16)$$

### 2. Beam splitter

A balanced beamsplitter is modeled by the two-mode matrix:

$$\mathbf{M}_{\text{bs}} = \frac{1}{\sqrt{2}} \begin{bmatrix} 1 & 0 & 1 & 0 \\ 0 & 1 & 0 & 1 \\ -1 & 0 & 1 & 0 \\ 0 & -1 & 0 & 1 \end{bmatrix} = \frac{1}{\sqrt{2}} \begin{bmatrix} \mathbf{1} & \mathbf{1} \\ -\mathbf{1} & \mathbf{1} \end{bmatrix}. \quad (17)$$

## D. Spectral densities

We define the symmetrized double-sided cross-correlation spectrum of a pair of quantum operators  $\hat{A}$  and  $\hat{B}$  by

$$\bar{S}_{AB}[\Omega] = \int_{-\infty}^{\infty} \frac{\langle \{\hat{A}^\dagger(t), \hat{B}(0)\} \rangle}{2} e^{i\Omega t} dt = \int_{-\infty}^{\infty} \frac{\langle \{\hat{A}^\dagger[\Omega], \hat{B}[\Omega']\} \rangle}{2} \frac{d\Omega'}{2\pi}. \quad (18)$$

Similarly, given a vector operator,  $\hat{\mathbf{A}}$ , we define the spectral density matrix  $\bar{\mathbf{S}}_{AA}[\Omega]$  by [3]

$$(\bar{\mathbf{S}}_{AA}[\Omega])_{ij} = \bar{S}_{A_i A_j}[\Omega]. \quad (19)$$

We call an operator  $\hat{\mathbf{A}}$  “weak-stationary” if it satisfies  $\langle \hat{A}_i(t) \hat{A}_j(t') \rangle = \langle \hat{A}_i(t - t') \hat{A}_j(0) \rangle \forall i, j$ . For weak-stationary observables  $\hat{X}, \hat{Y}$  spectral density has a simplified form

$$\bar{S}_{XY}[\Omega] = \frac{1}{4\pi\delta[0]} \langle \{\hat{X}[\Omega], \hat{Y}[\Omega]^\dagger\} \rangle \quad (20)$$

Using our conventions, the vacuum state has spectral density  $\bar{S}_{\text{vac}} = 1/2$ .

In practice, since all measurements are taken on a finite time interval, delta functions  $\delta[0]$  and integrals over all times  $\int_{-\infty}^{+\infty} dt$  should be understood as being limited in a finite experiment time interval  $[-T/2, T/2]$  with  $T \rightarrow +\infty$  the duration of the measurement. This way,

$$2\pi\delta[\omega] = \int_{-\infty}^{+\infty} e^{i\omega t} dt = \int_{-T/2}^{+T/2} e^{i\omega t} dt = T \text{sinc}\left(\frac{\omega T}{2}\right) \quad \text{i.e.} \quad \delta[0] \simeq \frac{1}{2\pi} \int_{-\infty}^{+\infty} dt \simeq \frac{T}{2\pi} \quad (21)$$

Therefore, defining finite-time Fourier transforms  $\hat{X}_T[\Omega] := \int_{-T/2}^{T/2} e^{-i\Omega t} \hat{X}(t) dt$  and similarly for  $\hat{Y}_T[\Omega]$ , eq. (20) reads

$$\bar{S}_{XY}[\Omega] = \frac{\langle \{ \hat{X}_T[\Omega], \hat{Y}_T[\Omega]^\dagger \} \rangle}{2T}. \quad (22)$$

### E. Some properties of $\text{rect}(x)$

In this section, we detail some properties of the box function  $\text{rect}(x)$  and define the normalization conventions we adopt for the box, triangle, and sinc functions.

We first recall the definition of the box function,

$$\text{rect}\left(\frac{x}{\Delta x}\right) := \begin{cases} 0 & \text{if } |x| > \Delta x/2 \\ 1 & \text{if } |x| \leq \Delta x/2 \end{cases}, \quad (23)$$

the triangle function,  $\text{tri}(x)$ ,

$$\text{tri}\left(\frac{x}{\Delta x}\right) := \begin{cases} 0 & \text{if } |x| > \Delta x \\ 1 - |x/\Delta x| & \text{if } |x| \leq \Delta x \end{cases} \quad (24)$$

and the sinc function,  $\text{sinc}(x)$ ,

$$\text{sinc}(x) := \frac{\sin(x)}{x}. \quad (25)$$

The sinc function has the property that  $\text{sinc}(0) = 1$ . We note that signal processing texts sometimes adopt different conventions in the definition of the sinc and tri functions, so it is important to remain consistent with the definitions chosen and be careful when referring to Fourier-transform tables to ensure they use the same conventions as we do here.

The rect and sinc functions are related by a Fourier transform:

$$\int_{-\infty}^{\infty} \frac{d\Omega}{2\pi} \text{rect}\left(\frac{\Omega}{\Delta\Omega}\right) e^{-i\Omega t} = \frac{1}{2\pi} \int_{-\Delta\Omega/2}^{\Delta\Omega/2} d\Omega e^{-i\Omega t} = \frac{\Delta\Omega}{2\pi} \text{sinc}\left(\frac{\Delta\Omega t}{2}\right), \quad (26)$$

such that

$$\begin{aligned} \int_{-\infty}^{\infty} \frac{d\Omega}{2\pi} \text{rect}\left(\frac{\Omega}{\Delta\Omega}\right) e^{-i\Omega t} &= \frac{\Delta\Omega}{2\pi} \text{sinc}\left(\frac{\Delta\Omega t}{2}\right) \\ \int_{-\infty}^{\infty} dt \frac{\Delta\Omega}{2\pi} \text{sinc}\left(\frac{\Delta\Omega t}{2}\right) e^{i\Omega t} &= \text{rect}\left(\frac{\Omega}{\Delta\Omega}\right). \end{aligned} \quad (27)$$

Taking  $H[\Omega] = \text{rect}((\Omega + \Omega_0)/\Delta\Omega) + \text{rect}((\Omega - \Omega_0)/\Delta\Omega)$ , the integrals  $\int_{-\infty}^{\infty} \frac{d\Omega'}{2\pi} H[\Omega'] H[\Omega - \Omega']$  and  $\int_{-\infty}^{\infty} \frac{d\Omega'}{2\pi} H[\Omega']$  naturally appear in the phase spectrum of an interferometer employing band-limited squeezed states:

$$\int_{-\infty}^{\infty} \frac{d\Omega'}{2\pi} H[\Omega'] H[\Omega - \Omega'] = \frac{\Delta\Omega}{\pi} \text{tri}\left(\frac{\Omega}{\Delta\Omega}\right) \quad (28)$$

and

$$\int_{-\infty}^{\infty} \frac{d\Omega'}{2\pi} H[\Omega'] = \frac{\Delta\Omega}{\pi}. \quad (29)$$

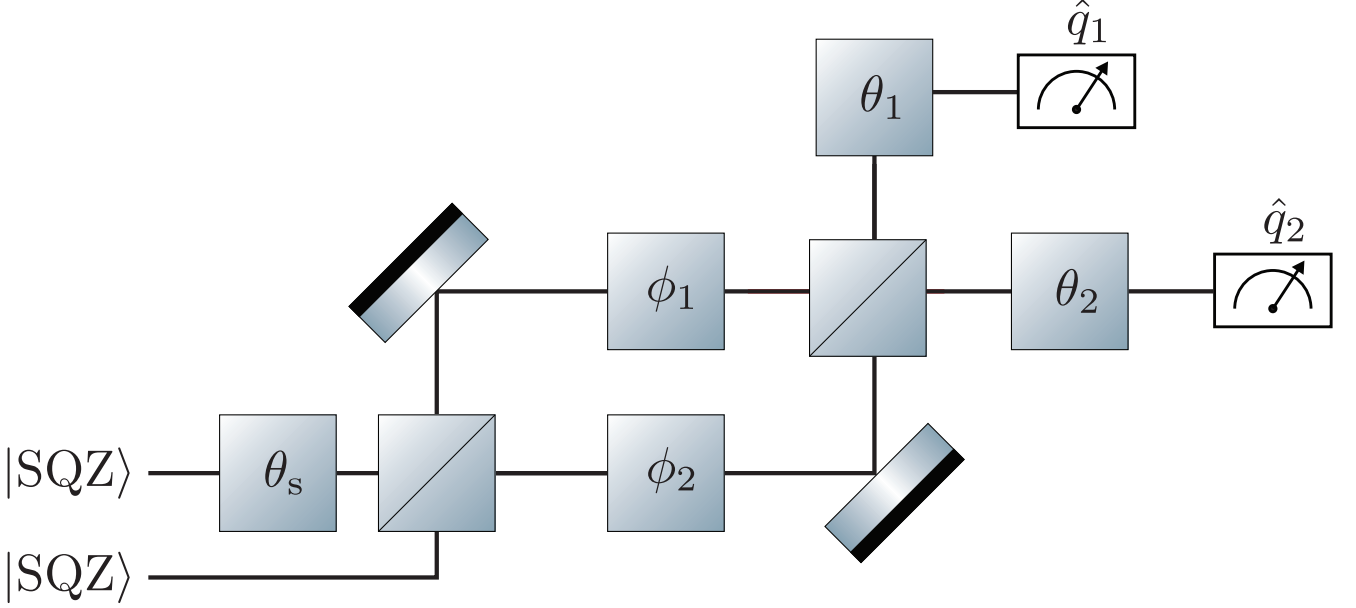

FIG. 1. A schematic showing an interferometer with a pair of squeezed states as inputs. A pair of squeezed states with a relative phase-angle  $\theta_s$  are launched into the interferometer. The arms of the interferometer receive phase-shifts  $\phi_1$  and  $\phi_2$ . A pair of homodyne detectors then measure the interferometer's output states at angles  $\theta_1$  and  $\theta_2$ . This last step is equivalent to first rotating the output states by phase-angles  $\theta_1$  and  $\theta_2$  and then measuring the position quadrature of each mode. The homodyne outputs are then subtracted and squared to derive information about the interferometer's differential phase,  $\phi_d = \phi_1 - \phi_2$ .

## II. THEORY: SPECTRAL QUANTUM CRAMER RAO BOUND FOR A MACH-ZEHNDER INTERFEROMETER

In this section we derive the spectral quantum Cramer-Rao bound for the Mach-Zehnder interferometer. Consider a system governed by the Hamiltonian  $\hat{H}(\delta\phi(t))$  where the time-varying signal  $\delta\phi(t)$  is to be estimated. We define the operator  $\hat{h}(t) = \hat{U}^\dagger(t)\partial_{\delta\phi}\hat{H}(\delta\phi(t))\hat{U}(t)$  “canonically associated” to  $\delta\phi(t)$  in the Heisenberg picture. Assuming that  $\delta\phi(t)$  is a zero-mean, weak-stationary random process with an uninformative prior and that  $\delta\tilde{\phi}(t)$  is an estimator of  $\delta\phi(t)$ , the spectral QCRB is (see [4] with  $\hbar = 1$ )

$$\bar{S}_{\delta\tilde{\phi}\delta\tilde{\phi}}[\Omega] \geq \frac{1}{4\bar{S}_{hh}[\Omega]}. \quad (30)$$

In the following sections, we express the evolution of the quantum states through the Mach-Zehnder interferometer to determine the expression of the generator  $\hat{h}(t)$ . We then compute its associated spectrum  $\bar{S}_{hh}[\Omega]$  for a two-mode input squeezed vacuum field, then for an input made of a coherent state in one mode and a squeezed vacuum in the other.

### A. Propagation of squeezed states through a Mach-Zehnder interferometer

The goal of this section is to explicitly express the generator  $\hat{h}(t)$  as a function of the quadrature operators injected at the input of the Mach-Zehnder. Figure 1 shows the experimental scheme. The transfer function from the input squeezed modes  $\hat{\mathbf{x}}^{\text{in}}$  to the readout of the homodyne detectors  $\hat{\mathbf{x}}^{\text{out}}$  is

$$\hat{\mathbf{x}}^{\text{out}}(t) = \mathbf{M}(t)\hat{\mathbf{x}}^{\text{in}}(t) = \mathbf{R}(\theta_1, \theta_2)\mathbf{M}_{\text{bs}}^T\mathbf{R}(\phi_1, \phi_2)\mathbf{M}_{\text{bs}}\mathbf{R}(0, \theta_s)\hat{\mathbf{x}}^{\text{in}}(t). \quad (31)$$

Equivalently,  $\mathbf{M}$  can be written, using the identities  $\mathbf{R}(a) + \mathbf{R}(b) = 2 \cos\left(\frac{a-b}{2}\right) \mathbf{R}\left(\frac{a+b}{2}\right)$  and  $\mathbf{R}(a) - \mathbf{R}(b) = 2 \sin\left(\frac{a-b}{2}\right) \mathbf{R}\left(\frac{a+b+\pi}{2}\right)$ :

$$\mathbf{M} = \begin{bmatrix} \cos\left(\frac{\phi_d}{2}\right) \mathbf{R}\left(\theta_1 + \frac{\phi_c}{2}\right) & \sin\left(\frac{\phi_d}{2}\right) \mathbf{R}\left(\theta_1 + \theta_s + \frac{\phi_c + \pi}{2}\right) \\ \sin\left(\frac{\phi_d}{2}\right) \mathbf{R}\left(\theta_2 + \frac{\phi_c + \pi}{2}\right) & \cos\left(\frac{\phi_d}{2}\right) \mathbf{R}\left(\theta_2 + \theta_s + \frac{\phi_c}{2}\right) \end{bmatrix} \quad (32)$$

where we have defined  $\phi_d = \phi_1 - \phi_2$  and  $\phi_c = \phi_1 + \phi_2$ . In the rest of the paper, we fix the setpoint of the interferometer such that

$$\phi_d = -\frac{\pi}{2} - \delta\phi(t), \quad \phi_c = 0, \quad \theta_s = 0, \quad \theta_1 = -\frac{\pi}{2}, \quad \theta_2 = 0. \quad (33)$$

In practice, we use feedback control to stabilize the system at this setpoint, as detailed in the main text, Methods, and Supplementary Information section IV. At this setpoint, the transfer function at lowest order is

$$\hat{\mathbf{x}}^{\text{out}}(t) = \left( \frac{1}{\sqrt{2}} \begin{bmatrix} 0 & 1 & -1 & 0 \\ -1 & 0 & 0 & -1 \\ 0 & 1 & 1 & 0 \\ -1 & 0 & 0 & 1 \end{bmatrix} + \frac{\delta\phi(t)}{2\sqrt{2}} \begin{bmatrix} 0 & -1 & -1 & 0 \\ 1 & 0 & 0 & -1 \\ 0 & 1 & -1 & 0 \\ -1 & 0 & 0 & -1 \end{bmatrix} + \mathcal{O}(\delta\phi^2) \right) \hat{\mathbf{x}}^{\text{in}}(t). \quad (34)$$

We denote these matrices by  $\mathbf{M}_0$  and  $\mathbf{M}_1$  such that

$$\hat{\mathbf{x}}^{\text{out}}(t) = \mathbf{M}_0 \hat{\mathbf{x}}^{\text{in}}(t) + \delta\phi(t) \mathbf{M}_1 \hat{\mathbf{x}}^{\text{in}}(t). \quad (35)$$

We further define the quadrature vector  $\hat{\mathbf{x}}^{(0)}(t) := \mathbf{M}_0 \hat{\mathbf{x}}^{\text{in}}(t)$  to be the output in the absence of any signal (i.e. when  $\delta\phi(t) = 0$ ). We can then rewrite eq. (35) in terms of  $\hat{\mathbf{x}}^{(0)}(t)$  as

$$\hat{\mathbf{x}}^{\text{out}}(t) = \hat{\mathbf{x}}^{(0)}(t) + \delta\phi(t) \mathbf{M}_1 \mathbf{M}_0^{-1} \hat{\mathbf{x}}^{(0)}(t), \quad (36)$$

This equation can be rewritten in the following form that allows us to identify the interaction Hamiltonian:

$$\hat{\mathbf{x}}^{\text{out}}(t) = \hat{\mathbf{x}}^{(0)}(t) + i \int_{-\infty}^t dt' \left[ \hat{V}(t'), \hat{\mathbf{x}}^{(0)}(t) \right] \quad (37)$$

where

$$\hat{V}(t) := \frac{\delta\phi}{2} \left( \hat{q}_1^{(0)}(t) \hat{p}_2^{(0)}(t) - \hat{p}_1^{(0)}(t) \hat{q}_2^{(0)}(t) \right) = \frac{\delta\phi}{2} \left( \hat{q}_1^{\text{in}}(t) \hat{q}_2^{\text{in}}(t) + \hat{p}_1^{\text{in}}(t) \hat{p}_2^{\text{in}}(t) \right). \quad (38)$$

We can finally identify the operator canonically associated with  $\delta\phi(t)$  as

$$\hat{h}(t) := \frac{\partial \hat{V}}{\partial \delta\phi} = \frac{1}{2} \left( \hat{q}_1^{\text{in}}(t) \hat{q}_2^{\text{in}}(t) + \hat{p}_1^{\text{in}}(t) \hat{p}_2^{\text{in}}(t) \right). \quad (39)$$

The input modes are uncorrelated so we have  $\langle \hat{h}(t) \rangle = 0$ .

## B. Spectral Quantum Cramer-Rao bound for two-mode squeezed field input

To determine the bound on phase estimation, we want to determine the PSD  $\bar{S}_{hh}[\Omega] = \frac{\langle \{\hat{h}[\Omega], \hat{h}[\Omega]^\dagger\} \rangle}{4\pi\delta[0]}$ . We first compute the Fourier transform of  $\hat{h}(t)$  using its definition eq. (39) and eq. (14):

$$\hat{h}[\Omega] = \frac{1}{2} \int_{-\infty}^{+\infty} \frac{d\Omega'}{2\pi} \left( \hat{q}_1^{\text{in}}[\Omega'] \hat{q}_2^{\text{in}}[\Omega - \Omega'] + \hat{p}_1^{\text{in}}[\Omega'] \hat{p}_2^{\text{in}}[\Omega - \Omega'] \right) \quad (40)$$

For now, we assume an ideal lossless system. Even in the ideal limit, the OPA must have a finite bandwidth or it would have an infinite output photon flux, which is unphysical. To model this, we take

$$\hat{x}_i^{\text{in}}[\Omega] = e^{\pm r[\Omega]} \hat{x}_i^{\text{vac}}[\Omega] := R_\pm[\Omega] \hat{x}_i^{\text{vac}}[\Omega], \quad R_\pm[\Omega] \in \mathbb{R}. \quad (41)$$

The + corresponds to the anti-squeezed  $q$  quadratures and the - corresponds to the squeezed  $p$  quadratures. Injecting this into the previous equation yields

$$\hat{h}[\Omega] = \frac{1}{2} \int_{-\infty}^{+\infty} \frac{d\Omega'}{2\pi} (R_+[\Omega'] R_+[\Omega - \Omega'] \hat{q}_1^{\text{vac}}[\Omega'] \hat{q}_2^{\text{vac}}[\Omega - \Omega'] + R_-[\Omega'] R_-[\Omega - \Omega'] \hat{p}_1^{\text{vac}}[\Omega'] \hat{p}_2^{\text{vac}}[\Omega - \Omega']). \quad (42)$$

Its spectral density is thus

$$\begin{aligned} \bar{S}_{hh}[\Omega] = \frac{1}{16\pi\delta[0]} \iint_{-\infty}^{+\infty} \frac{d\Omega' d\Omega''}{4\pi^2} & (R_+[\Omega'] R_+[\Omega - \Omega'] R_+[\Omega''] R_+[\Omega - \Omega''] \langle \{ \hat{q}_1^{\text{vac}}[\Omega'] \hat{q}_2^{\text{vac}}[\Omega - \Omega'], \hat{q}_1^{\text{vac}}[\Omega''] \hat{q}_2^{\text{vac}}[\Omega - \Omega'']^\dagger \} \rangle \\ & + R_+[\Omega'] R_+[\Omega - \Omega'] R_-[\Omega''] R_-[\Omega - \Omega''] \langle \{ \hat{q}_1^{\text{vac}}[\Omega'] \hat{q}_2^{\text{vac}}[\Omega - \Omega'], \hat{p}_1^{\text{vac}}[\Omega''] \hat{p}_2^{\text{vac}}[\Omega - \Omega'']^\dagger \} \rangle \\ & + R_-[\Omega'] R_-[\Omega - \Omega'] R_+[\Omega''] R_+[\Omega - \Omega''] \langle \{ \hat{p}_1^{\text{vac}}[\Omega'] \hat{p}_2^{\text{vac}}[\Omega - \Omega'], \hat{q}_1^{\text{vac}}[\Omega''] \hat{q}_2^{\text{vac}}[\Omega - \Omega'']^\dagger \} \rangle \\ & + R_-[\Omega'] R_-[\Omega - \Omega'] R_-[\Omega''] R_-[\Omega - \Omega''] \langle \{ \hat{p}_1^{\text{vac}}[\Omega'] \hat{p}_2^{\text{vac}}[\Omega - \Omega'], \hat{p}_1^{\text{vac}}[\Omega''] \hat{p}_2^{\text{vac}}[\Omega - \Omega'']^\dagger \} \rangle). \end{aligned} \quad (43)$$

We compute each anti-commutator by separating the quadratures pertaining to each mode (as they commute between modes) and use the unsymmetrized two-point averages:

$$\langle \hat{q}_1^{\text{vac}}[\omega] \hat{q}_1^{\text{vac}}[\omega']^\dagger \rangle = \langle \hat{p}_1^{\text{vac}}[\omega] \hat{p}_1^{\text{vac}}[\omega']^\dagger \rangle = \pi \delta[\omega - \omega'] \quad (44)$$

$$\langle \hat{q}_1^{\text{vac}}[\omega] \hat{p}_1^{\text{vac}}[\omega']^\dagger \rangle = -\langle \hat{p}_1^{\text{vac}}[\omega] \hat{q}_1^{\text{vac}}[\omega']^\dagger \rangle = i\pi \delta[\omega - \omega'], \quad (45)$$

and similarly for mode 2. Thus,

$$\begin{aligned} \langle \{ \hat{q}_1^{\text{vac}}[\Omega'] \hat{q}_2^{\text{vac}}[\Omega - \Omega'], \hat{q}_1^{\text{vac}}[\Omega''] \hat{q}_2^{\text{vac}}[\Omega - \Omega'']^\dagger \} \rangle &= \langle \{ \hat{p}_1^{\text{vac}}[\Omega'] \hat{p}_2^{\text{vac}}[\Omega - \Omega'], \hat{p}_1^{\text{vac}}[\Omega''] \hat{p}_2^{\text{vac}}[\Omega - \Omega'']^\dagger \} \rangle = 2\pi^2 \delta[\Omega' - \Omega'']^2 \\ \langle \{ \hat{q}_1^{\text{vac}}[\Omega'] \hat{q}_2^{\text{vac}}[\Omega - \Omega'], \hat{p}_1^{\text{vac}}[\Omega''] \hat{p}_2^{\text{vac}}[\Omega - \Omega'']^\dagger \} \rangle &= \langle \{ \hat{p}_1^{\text{vac}}[\Omega'] \hat{p}_2^{\text{vac}}[\Omega - \Omega'], \hat{q}_1^{\text{vac}}[\Omega''] \hat{q}_2^{\text{vac}}[\Omega - \Omega'']^\dagger \} \rangle = -2\pi^2 \delta[\Omega' - \Omega'']^2. \end{aligned} \quad (46)$$

This simplifies the spectral density into

$$\bar{S}_{hh}[\Omega] = \frac{1}{32\pi} \int_{-\infty}^{+\infty} d\Omega' (R_+[\Omega']^2 R_+[\Omega - \Omega']^2 + R_-[\Omega']^2 R_-[\Omega - \Omega']^2 - 2R_+[\Omega'] R_+[\Omega - \Omega'] R_-[\Omega'] R_-[\Omega - \Omega']) \quad (47)$$

$$= \frac{1}{32\pi} \int_{-\infty}^{+\infty} d\Omega' (R_+[\Omega'] R_+[\Omega - \Omega'] - R_-[\Omega'] R_-[\Omega - \Omega'])^2. \quad (48)$$

We now assume that we have squeezing in a bandwidth  $\Delta\Omega$  centered around the frequency  $\Omega_0$ . With this assumption,  $r[\Omega]$  has the form

$$r[\Omega] = \begin{cases} r & \text{if } |\Omega + \Omega_0| \leq \Delta\Omega/2 \text{ or } |\Omega - \Omega_0| \leq \Delta\Omega/2 \\ 0 & \text{otherwise} \end{cases}. \quad (49)$$

With this form for  $r[\Omega]$ , we have

$$R_\pm[\Omega] = 1 + (e^{\pm r} - 1)H[\Omega], \quad (50)$$

where  $H[\Omega] = \text{rect}\left(\frac{\Omega - \Omega_0}{\Delta\Omega}\right) + \text{rect}\left(\frac{\Omega + \Omega_0}{\Delta\Omega}\right)$ . Note that because  $H[\Omega]^2 = H[\Omega]$  (assuming that  $\Omega_0 \geq \Delta\Omega/2$ , as is always the case physically), we have that  $R_\pm[\Omega]^2 = 1 + (e^{\pm 2r} - 1)H[\Omega]$ . Thus, using eqs. (28) and (29) we get

$$\bar{S}_{hh}[\Omega] = \frac{\Delta\Omega}{8\pi} \left[ (e^r - e^{-r})^2 + \frac{(e^{2r} - 1)^2 + (e^{-2r} - 1)^2}{2} \text{tri}\left(\frac{\Omega}{\Delta\Omega}\right) \right] \underset{\Omega \ll \Delta\Omega}{=} \frac{\Delta\Omega}{4\pi} \sinh^2(2r) \quad (51)$$

This yields a first form of the spectral QCRB:

$$\bar{S}_{\delta\tilde{\phi}\delta\tilde{\phi}}[\Omega] \geq \frac{\pi}{\Delta\Omega \sinh^2(2r)} = \frac{\pi}{\Delta\Omega n(n+2)} \quad (52)$$

for signals well below the bandwidth of the of squeezed field  $\Omega \ll \Delta\Omega$ , where  $n = 2 \sinh^2(r)$  is the number of photons per mode.

It is possible to express this directly as a function of the photon flux, to explicitly see that Heisenberg scaling is achieved. The mean photon flux  $\mathcal{N}$  (in photons per second) for a single mode is given by

$$\mathcal{N} = \int_{-\infty}^{+\infty} \frac{d\Omega}{2\pi} \langle \hat{a}[\Omega]^\dagger \hat{a}[\Omega] \rangle = \frac{1}{2} \int_{-\infty}^{\infty} \frac{d\Omega}{2\pi} (\bar{S}_{qq}[\Omega] + \bar{S}_{pp}[\Omega] - 1), \quad (53)$$

so the mean total photon flux from a pair of squeezed states with squeezing parameter  $r[\Omega]$  with the functional form given in eq. (49) is

$$\begin{aligned} \mathcal{N} &= \frac{1}{2} \int_{-\infty}^{\infty} \frac{d\Omega}{2\pi} (\bar{S}_{qq}^1[\Omega] + \bar{S}_{pp}^1[\Omega] + \bar{S}_{qq}^2[\Omega] + \bar{S}_{pp}^2[\Omega] - 2) \\ &= \int_{-\infty}^{\infty} \frac{d\Omega}{2\pi} (\bar{S}_{qq}^1[\Omega] + \bar{S}_{pp}^1[\Omega] - 1) \\ &= \frac{2\Delta\Omega \sinh^2(r)}{\pi}. \end{aligned} \quad (54)$$

Using  $\sinh^2(2r) = 4\sinh^2(r)(\sinh^2(r) + 1)$ , we find

$$\bar{S}_{\delta\phi\delta\phi}[\Omega] \geq \frac{\Delta\Omega}{\pi\mathcal{N}(\mathcal{N} + \frac{2\Delta\Omega}{\pi})} \quad (55)$$

We see that at constant bandwidth, this scales inversely with the photon flux for  $\mathcal{N}/\Delta\Omega \gg 1$ . In this limit, the right hand side is  $\approx \frac{\Delta\Omega}{\pi} \frac{1}{\mathcal{N}^2}$ , indicating that a measurement saturating the spectral QCRB achieves Heisenberg scaling.

### C. Spectral Quantum Cramer-Rao bound for a coherent and squeezed vacuum input

To understand the quantum advantage of an interferometer with a squeezed state injected into each input, it is interesting to compute the spectral QCRB for an interferometer with a coherent state injected into one input and a squeezed state injected into the other. For such an interferometer, the input quadrature operators are related to the vacuum quadrature operators by

$$\begin{aligned} \hat{q}_1^{\text{in}}[\Omega] &= \bar{q} \cdot 2\pi\delta[\Omega] + \hat{q}_1^{\text{vac}}[\Omega] \\ \hat{p}_1^{\text{in}}[\Omega] &= \hat{p}_1^{\text{vac}}[\Omega] \\ \hat{x}_2^{\text{in}}[\Omega] &= e^{\pm r[\Omega]} \hat{x}_2^{\text{vac}}[\Omega] := R_{\pm}[\Omega] \hat{x}_2^{\text{vac}}[\Omega]. \end{aligned} \quad (56)$$

The generator of the phase  $\hat{h}[\Omega]$  reads, according to eq. (40)

$$\hat{h}[\Omega] = \frac{\bar{q}}{2} R_+[\Omega] \hat{q}_2^{\text{vac}}[\Omega] + \frac{1}{2} \int_{-\infty}^{+\infty} \frac{d\Omega'}{2\pi} (R_+[\Omega - \Omega'] \hat{q}_1^{\text{vac}}[\Omega'] \hat{q}_2^{\text{vac}}[\Omega - \Omega'] + R_-[\Omega - \Omega'] \hat{p}_1^{\text{vac}}[\Omega'] \hat{p}_2^{\text{vac}}[\Omega - \Omega']) \quad (57)$$

To compute the spectral density  $\bar{S}_{hh}[\Omega]$ , we follow a similar approach as in the previous section. Using the anti-commutators of eq. (46), we find

$$\bar{S}_{hh}[\Omega] = \frac{\bar{q}^2}{8} R_+[\Omega]^2 + \frac{1}{32\pi} \int_{-\infty}^{+\infty} d\Omega' R_+[\Omega']^2 + R_-[\Omega']^2 - 2R_+[\Omega'] R_-[\Omega'] \quad (58)$$

This last integral evaluates to  $8\Delta\Omega \sinh^2(r)$ , from which we deduce the spectral density when  $H[\Omega] = 1$  (that is, for  $|\Omega - \Omega_0| < \Delta\Omega/2$ )

$$\bar{S}_{hh}[\Omega] = \frac{\bar{q}^2 e^{2r}}{8} + \frac{\Delta\Omega}{4\pi} \sinh^2(r), \quad (59)$$

such that the spectral QCRB reads

$$\bar{S}_{\delta\phi\delta\phi}[\Omega] \geq \frac{1}{4\bar{S}_{hh}[\Omega]} = \frac{2}{\bar{q}^2 e^{2r} + \frac{2\Delta\Omega}{\pi} \sinh^2(r)}. \quad (60)$$



We will now relate this bound to the photon number flux into the interferometer. From eq. (53), the number flux into the coherent state's input is

$$\mathcal{N}_1(t) = \frac{1}{2} \int_{-\infty}^{\infty} \frac{d\Omega}{2\pi} \left( \bar{S}_{qq}^{\text{in},1}[\Omega] + \bar{S}_{pp}^{\text{in},1}[\Omega] - 1 \right) = \frac{1}{2} \bar{q}^2. \quad (61)$$

Assuming the state incident on the second port is a squeezed state with squeezing parameter  $r$  and bandwidth  $\Delta\Omega$ , the number flux in the squeezed state input is

$$\mathcal{N}_2(t) = \frac{\Delta\Omega \sinh^2(r)}{\pi}. \quad (62)$$

Solving this for  $e^{2r}$ , we find

$$e^{2r} = 1 + \frac{2\pi\mathcal{N}_2}{\Delta\Omega} + \sqrt{\frac{4\pi\mathcal{N}_2}{\Delta\Omega} \left( 1 + \frac{\pi\mathcal{N}_2}{\Delta\Omega} \right)} = 2 + \frac{4\pi\mathcal{N}_2}{\Delta\Omega} + \mathcal{O}\left(\frac{\Delta\Omega}{\mathcal{N}_2}\right), \quad (63)$$

such that the bound on the PSD of the phase estimator is

$$\bar{S}_{\delta\tilde{\phi}\delta\tilde{\phi}}[\Omega] \geq \frac{1}{\mathcal{N}_1 \left( 1 + \frac{2\pi\mathcal{N}_2}{\Delta\Omega} + \sqrt{\frac{4\pi\mathcal{N}_2}{\Delta\Omega} \left( 1 + \frac{\pi\mathcal{N}_2}{\Delta\Omega} \right)} \right) + \mathcal{N}_2} \approx \frac{1}{2\mathcal{N}_1 + \mathcal{N}_2 + \frac{4\pi\mathcal{N}_1\mathcal{N}_2}{\Delta\Omega}}. \quad (64)$$

The approximation holds when  $\mathcal{N}_2/\Delta\Omega \gg 1$ . If we inject an equal number of photons into each input, we have  $\mathcal{N}_1 = \mathcal{N}_2 = \mathcal{N}/2$  and

$$\bar{S}_{\delta\tilde{\phi}\delta\tilde{\phi}}[\Omega] \gtrsim \frac{\Delta\Omega}{\pi} \frac{1}{\mathcal{N} \left( \mathcal{N} + \frac{3\Delta\Omega}{2\pi} \right)}. \quad (65)$$

On the other hand, if the second mode is in a vacuum state, then we have

$$\bar{S}_{\delta\tilde{\phi}\delta\tilde{\phi}}[\Omega] \geq \frac{1}{\mathcal{N}}, \quad (66)$$

where  $\mathcal{N} = \mathcal{N}_1$  here since all of the photons are in the first mode. This is the expected limit for interferometric sensitivity given by shot noise, often referred to as the standard quantum limit.

We now make several observations regarding eqs. (55), (65) and (66). First, we see that the schemes with one or two squeezed states parametrically evade the shot noise bound. Second, the scheme with a coherent state and a squeezed state and the scheme with two squeezed states both achieve Heisenberg scaling, although the latter is always slightly more sensitive. Third, the spectral regions of maximal sensitivity for the two squeezed state scheme and the squeezed and coherent state scheme do not overlap in general. The scheme with two squeezed states is always maximally sensitive at low frequencies, even if the squeezed states involved are only squeezed at high frequencies. On the other hand, the maximally sensitive region of the squeezed and coherent scheme is exactly the region where there is maximal squeezing.

Typical interferometers with coherent states on one of their inputs, such as LIGO, are operated on a dark fringe and are read out by a single homodyne detector, set to measure the phase quadrature. The mean value of the output phase quadrature is  $\langle \hat{p}^{\text{out}}(t) \rangle = \bar{q} \sin\left(\frac{\delta\phi(t)}{2}\right) \approx \frac{\bar{q}\delta\phi(t)}{2}$ , such that  $\delta\tilde{\phi} = 2\hat{p}^{\text{out}}/\bar{q}$ . Since the other input is squeezed, the output phase quadrature PSD, in the absence of a signal, is  $\bar{S}_{pp}^{\text{out}}[\Omega] = e^{2r[\Omega]}/2$ , such that the estimator PSD is

$$\bar{S}_{\delta\tilde{\phi}\delta\tilde{\phi}}[\Omega] = \frac{2}{\bar{q}^2 e^{2r[\Omega]}} \approx \frac{\Delta\Omega}{\pi} \frac{1}{\mathcal{N} \left( \mathcal{N} + \frac{\Delta\Omega}{\pi} \right)}, \quad (67)$$

where the approximation is the same as that made in eq. (63), which led to eq. (65). Comparing eq. (65) with eq. (67), we see that the standard homodyne detection scheme is sub-optimal. Thus, not only is interferometric phase detection with a squeezed and a coherent state sub-optimal in the sense that its spectral QCRB is worse than that for a pair of squeezed states, but also in that standard measurement techniques do not saturate this spectral QCRB.

### III. OPTIMAL ESTIMATOR

In this section we construct an optimal phase estimator that reaches the spectral QCRB presented in eq. (55). The interferometer's input-output relation is given by eq. (35), from which we find the expression of the two quadratures that are read out by the homodyne detectors:

$$\begin{aligned} \hat{q}_1^{\text{out}}(t) &= \frac{1}{\sqrt{2}} \left( \hat{p}_1^{\text{in}}(t) - \hat{q}_2^{\text{in}}(t) \right) - \frac{\delta\phi(t)}{2\sqrt{2}} \left( \hat{p}_1^{\text{in}}(t) + \hat{q}_2^{\text{in}}(t) \right) \\ \hat{q}_2^{\text{out}}(t) &= \frac{1}{\sqrt{2}} \left( \hat{p}_1^{\text{in}}(t) + \hat{q}_2^{\text{in}}(t) \right) + \frac{\delta\phi(t)}{2\sqrt{2}} \left( \hat{p}_1^{\text{in}}(t) - \hat{q}_2^{\text{in}}(t) \right). \end{aligned} \quad (68)$$

Evidently, these output quadratures commute because they belong to different spatial free modes. Thus they represent a pair of simultaneously measurable quantities.

We would like to estimate the phase spectrum from the variances of these output quadratures. As a first step, we compute the autocorrelation of the input quadratures assuming that the OPA generating our squeezing is broadband with squeezing parameter  $r$  and a total transmissivity  $\eta$  such that

$$\hat{x}_i^{\text{in}}[\Omega] = \eta e^{\pm r} \hat{x}_i^{\text{vac}}[\Omega] + \sqrt{1 - \eta^2} \hat{x}_i^{\text{N}}[\Omega]. \quad (69)$$

From this, we compute

$$\begin{aligned} \langle \hat{x}_i^{\text{in}}(t) \hat{x}_i^{\text{in}}(t') \rangle &= \frac{1}{2} \left( \eta^2 e^{\pm 2r} + 1 - \eta^2 \right) \delta(t - t') \\ &:= V_{\pm} \delta(t - t'), \end{aligned} \quad (70)$$

or in the frequency domain

$$\langle \hat{x}_i^{\text{in}}[\Omega] \hat{x}_i^{\text{in}}[\Omega'] \rangle := 2\pi V_{\pm} \delta[\Omega + \Omega']. \quad (71)$$

Here, we have defined the quadrature variances  $V_{\pm} := \frac{1}{2} \left( \eta^2 e^{\pm 2r} + 1 - \eta^2 \right)$ . In the absence of losses, when  $\eta = 1$ , these are  $V_{\pm} = e^{\pm 2r}/2$ .

We would like to construct our time-domain phase-estimator from the quadrature variances at the same point in time. However, from eqs. (68) and (70), we see that these variances are infinite, even in the absence of squeezing when  $r = 0$ . Fortunately, we cannot observe these variances directly, only a filtered version of them which enforces a high-frequency cutoff and possibly a low-frequency cutoff as well. In this case, we directly measure the quadratures  $\tilde{x}_i^{\text{out}}$ , through the filter  $H[\Omega]$  as

$$\tilde{x}_i^{\text{out}}[\Omega] = H[\Omega] \hat{x}_i^{\text{out}}[\Omega]. \quad (72)$$

We would like to construct an estimator of  $\delta\phi(t)$  from  $\tilde{q}_1^{\text{out}}(t)$  and  $\tilde{q}_2^{\text{out}}(t)$ . The mean values of these operators are zero. Their variances are nonzero and are given by

$$\begin{aligned} \langle \tilde{q}_1^{\text{out}}(t)^2 \rangle &= \int_{-\infty}^{\infty} dt' H(t')^2 \left( \frac{1}{2} (V_+ + V_-) + \frac{\delta\phi(t - t')}{2} (V_+ - V_-) \right) + \mathcal{O}(\delta\phi(t)^2) \\ \langle \tilde{q}_2^{\text{out}}(t)^2 \rangle &= \int_{-\infty}^{\infty} dt' H(t')^2 \left( \frac{1}{2} (V_+ + V_-) - \frac{\delta\phi(t - t')}{2} (V_+ - V_-) \right) + \mathcal{O}(\delta\phi(t)^2), \end{aligned} \quad (73)$$

and their difference at leading order in  $\delta\phi(t)$  is

$$\langle \tilde{q}_1^{\text{out}}(t)^2 \rangle - \langle \tilde{q}_2^{\text{out}}(t)^2 \rangle = (V_+ - V_-) \int_{-\infty}^{\infty} dt' H(t')^2 \delta\phi(t - t'). \quad (74)$$

We choose our estimator,  $\delta\tilde{\phi}(t)$ , of  $\delta\phi(t)$  to be

$$\delta\tilde{\phi}(t) = \int_{-\infty}^{\infty} \frac{d\Omega}{2\pi} e^{-i\Omega t} \frac{\int_{-\infty}^{\infty} dt' e^{i\Omega t'} \left( \tilde{q}_1^{\text{out}}(t')^2 - \tilde{q}_2^{\text{out}}(t')^2 \right)}{(V_+ - V_-) H^2[\Omega]}, \quad (75)$$

where  $H^2[\Omega]$  is the Fourier transform of  $H(t)^2$ . For frequencies substantially less than the squeezing bandwidth, i.e for  $\Omega \ll \Delta\Omega$ , we have  $H^2[\Omega] = (\Delta\Omega/\pi)\text{tri}(\Omega/\Delta\Omega) \approx \Delta\Omega/\pi$  and the estimator is approximated by

$$\delta\tilde{\phi}(t) \approx \frac{\tilde{q}_1^{\text{out}}(t)^2 - \tilde{q}_2^{\text{out}}(t)^2}{(V_+ - V_-)(\Delta\Omega/\pi)}. \quad (76)$$

As discussed in the main text, this approximate estimator can be understood as subtracting the rectified and filtered homodyne voltages and multiplying by an appropriate scaling factor determined by the bandwidth of the filter applied to the homodyne voltages and the squeezing level.

### A. Proof that the estimator is unbiased

We can see that this estimator is locally unbiased by computing its expectation value using eq. (74) and eq. (14). At leading order, we find

$$\langle \delta\tilde{\phi}(t) \rangle = \int_{-\infty}^{\infty} \frac{d\Omega}{2\pi} e^{-i\Omega t} \delta\phi[\Omega] = \delta\phi(t). \quad (77)$$

We note that in our measurement, we are estimating a random process  $\delta\phi(t)$ , rather than a fixed but unknown random variable, so the spectral QCRB holds for all estimators, not only unbiased estimators [4]. However, the fact that our estimator is unbiased is still important, as it tells us that the estimator recovers the random process in expectation.

### B. Proof of saturability of spectral QCRB

The spectrum of the estimation error in presence of the signal,  $\bar{S}_{\delta\tilde{\phi}\delta\tilde{\phi}}[\Omega]$ , corresponds to the power spectral density of  $\delta\tilde{\phi}(t)$  when no signal is present. In other words,  $\bar{S}_{\delta\tilde{\phi}\delta\tilde{\phi}}[\Omega] = \frac{1}{4\pi\delta[0]} \langle \{\delta\tilde{\phi}[\Omega], \delta\tilde{\phi}[\Omega]^\dagger\} \rangle|_{\delta\phi=0}$ . Note that the Fourier transform of  $\delta\tilde{\phi}$  is

$$\delta\tilde{\phi}[\Omega] = \frac{1}{(V_+ - V_-)H^2[\Omega]} \int \frac{d\Omega'}{2\pi} H[\Omega'] H[\Omega - \Omega'] \left( \tilde{q}_1^{\text{out}}[\Omega'] \tilde{q}_1^{\text{out}}[\Omega - \Omega'] - \tilde{q}_2^{\text{out}}[\Omega'] \tilde{q}_2^{\text{out}}[\Omega - \Omega'] \right), \quad (78)$$

which can be expressed as a function of the input quadratures as

$$\delta\tilde{\phi}[\Omega]|_{\delta\phi=0} = \frac{-1}{(V_+ - V_-)H^2[\Omega]} \int \frac{d\Omega'}{\pi} H[\Omega'] H[\Omega - \Omega'] \hat{p}_1^{\text{in}}[\Omega'] \hat{q}_2^{\text{in}}[\Omega - \Omega']. \quad (79)$$

The spectrum is

$$\bar{S}_{\delta\tilde{\phi}\delta\tilde{\phi}}[\Omega] = \frac{1}{4\pi^3\delta[0](V_+ - V_-)^2|H^2[\Omega]|^2} \iint_{-\infty}^{+\infty} d\Omega' d\Omega'' H[\Omega'] H[\Omega - \Omega'] H[\Omega'']^* H[\Omega - \Omega'']^* \times \quad (80)$$

$$\langle \{\hat{p}_1^{\text{in}}[\Omega'] \hat{q}_2^{\text{in}}[\Omega - \Omega'], \hat{p}_1^{\text{in}}[\Omega'']^\dagger \hat{q}_2^{\text{in}}[\Omega - \Omega'']^\dagger\} \rangle. \quad (81)$$

Notice that the anticommutator can be explicitly computed using eq. (71) and the fact that quadratures of different modes commute:

$$\langle \{\hat{p}_1^{\text{in}}[\Omega'] \hat{q}_2^{\text{in}}[\Omega - \Omega'], \hat{p}_1^{\text{in}}[\Omega'']^\dagger \hat{q}_2^{\text{in}}[\Omega - \Omega'']^\dagger\} \rangle = \langle \hat{p}_1^{\text{in}}[\Omega'] \hat{p}_1^{\text{in}}[\Omega'']^\dagger \rangle \langle \hat{q}_2^{\text{in}}[\Omega - \Omega'] \hat{q}_2^{\text{in}}[\Omega - \Omega'']^\dagger \rangle \quad (82)$$

$$+ \langle \hat{p}_1^{\text{in}}[\Omega'']^\dagger \hat{p}_1^{\text{in}}[\Omega'] \rangle \langle \hat{q}_2^{\text{in}}[\Omega - \Omega'']^\dagger \hat{q}_2^{\text{in}}[\Omega - \Omega'] \rangle \quad (83)$$

$$= (2\pi)^2 V_+ V_- \delta[\Omega' - \Omega'']^2 + (2\pi)^2 V_+ V_- \delta[\Omega' - \Omega'']^2 \quad (84)$$

$$= 8\pi^2 V_+ V_- \delta[\Omega' - \Omega'']^2. \quad (85)$$

Plugging this into the previous expression yields

$$\bar{S}_{\delta\tilde{\phi}\delta\tilde{\phi}}[\Omega] = \frac{2V_+ V_-}{\pi(V_+ - V_-)^2|H^2[\Omega]|^2} \int_{-\infty}^{+\infty} d\Omega' |H[\Omega']|^2 |H[\Omega - \Omega']|^2. \quad (86)$$

We now make an explicit choice of this filter function and take it to be  $H[\Omega] = \text{rect}((\Omega + \Omega_0)/\Delta\Omega) + \text{rect}((\Omega - \Omega_0)/\Delta\Omega)$ . According to eq. (28), we then have  $H^2[\Omega] = \int \frac{d\Omega'}{2\pi} H[\Omega'] H[\Omega - \Omega'] = \Delta\Omega/\pi + \mathcal{O}((\Omega/\Delta\Omega)^2)$  and since  $|H[\Omega]|^2 = H[\Omega]$ , the integral evaluates to  $2\Delta\Omega + \mathcal{O}((\Omega/\Delta\Omega)^2)$ . Finally, at lowest order,

$$\bar{S}_{\delta\phi\delta\phi}[\Omega] = \frac{4\pi V_+ V_-}{(V_+ - V_-)^2 \Delta\Omega}. \quad (87)$$

In the lossless case, we have  $V_{\pm} = e^{\pm 2r}/2$  and

$$\bar{S}_{\delta\phi\delta\phi}[\Omega] = \frac{\pi}{\Delta\Omega} \frac{1}{\sinh^2(2r)}, \quad (88)$$

which is in agreement with the analysis in section II B, particularly eq. (52), thus showing that the spectral QCRB is attained.

For nonzero experimental losses, we have

$$\bar{S}_{\delta\phi\delta\phi}[\Omega] = \frac{1 + 2L(1-L)^2 n}{\frac{\Delta\Omega}{\pi}(1-L)^3 n((1-L)n + 2)}, \quad (89)$$

where  $L := \sqrt{1 - \eta^2}$  is the loss on the incident squeezed states. We can verify that this reduces to the lossless limit for  $L = 0$ .

### C. Proof that the optimal estimator corresponds to the MLE

From the most general expression of the transfer function of the MZI, it's possible to obtain a matrix form of the propagation of the quantum noise:

$$\mathbf{q}^{\text{out}}(t) = \begin{bmatrix} \hat{q}_1^{\text{out}}(t) \\ \hat{q}_2^{\text{out}}(t) \end{bmatrix} = \mathbf{M}_q(t) \mathbf{q}^{\text{in}}(t) = \begin{bmatrix} \cos\left(\frac{\delta\phi(t)}{2} + \frac{\pi}{4}\right) & -\cos\left(\frac{\delta\phi(t)}{2} - \frac{\pi}{4}\right) \\ \cos\left(\frac{\delta\phi(t)}{2} - \frac{\pi}{4}\right) & \cos\left(\frac{\delta\phi(t)}{2} + \frac{\pi}{4}\right) \end{bmatrix} \begin{bmatrix} \hat{p}_1^{\text{in}}(t) \\ \hat{q}_2^{\text{in}}(t) \end{bmatrix}. \quad (90)$$

This means that the two-point time covariance is a function of the input covariance:

$$\mathbf{V}^{\text{out}}(t, t') := \langle \mathbf{q}^{\text{out}}(t) \mathbf{q}^{\text{out}}(t')^\dagger \rangle = \mathbf{M}_q(t) \mathbf{V}^{\text{in}}(t, t') \mathbf{M}_q(t')^\dagger. \quad (91)$$

Since  $\mathbf{V}^{\text{in}}(t, t') = \begin{bmatrix} V_- & 0 \\ 0 & V_+ \end{bmatrix} \delta(t - t')$  (according to eq. (70)) we get

$$\mathbf{V}^{\text{out}}(t, t') = \left( \frac{V_+ + V_-}{2} \mathbf{1} + \frac{V_+ - V_-}{2} \begin{bmatrix} \sin \delta\phi(t) & -\cos \delta\phi(t) \\ -\cos \delta\phi(t) & -\sin \delta\phi(t) \end{bmatrix} \right) \delta(t - t') =: \mathbf{V}(t) \delta(t - t'). \quad (92)$$

We only have access to the filtered noise, which we recall as being  $\tilde{q}_i(t) = \int H(t') \hat{q}_i^{\text{out}}(t - t') dt'$ . The associated two-point covariance is

$$\tilde{V}_{ij}(t_1, t_2) = \iint dt' dt'' H(t_1 - t') H(t_2 - t'') V_{ij}(t') \delta(t' - t'') = \int dt' H(t_1 - t') H(t_2 - t') V_{ij}(t'). \quad (93)$$

Assume that we are sampling data at times  $t_k$ ,  $k \in \mathbb{Z}$ , in such a way that the samples at different times are uncorrelated. This means that, for any  $k, k' \in \mathbb{Z}$ , and for any  $i, j \in \{1, 2\}$ ,  $\tilde{V}_{ij}(t_k, t_{k'}) = V_{ij}(t_k) \frac{\Delta\Omega}{\pi} \delta_{k, k'}$ . For example, this can be realized with the proposed shape for the filter  $H[\Omega] = \text{rect}((\Omega + \Omega_0)/\Delta\Omega) + \text{rect}((\Omega - \Omega_0)/\Delta\Omega)$  if we assume its bandwidth  $\Delta\Omega$  to be much larger than the characteristic frequency of  $\delta\phi$  (which is the case in practice) and if we sample at times  $t_k = 2\pi k/\Delta\Omega$ .

Under this model, our data is made of the samples  $\{\tilde{q}_1(t_k), \tilde{q}_2(t_k)\}_{k \in \mathbb{Z}}$  where the samples at different times are independent and follow gaussian distributions:  $(\tilde{q}_1(t_k), \tilde{q}_2(t_k)) \sim \mathcal{N}(0, \tilde{\mathbf{V}}(t_k))$  where we denote  $\tilde{\mathbf{V}}(t_k) = \mathbf{V}(t_k) \Delta\Omega/\pi$ . The corresponding joint probability distribution is

$$p(\tilde{q}_1(t_k), \tilde{q}_2(t_k)) = \frac{1}{2\pi \sqrt{|\tilde{\mathbf{V}}|}} \exp \left( -\frac{\tilde{q}_1(t_k)^2 \tilde{V}_{22}(t_k) + \tilde{q}_2(t_k)^2 \tilde{V}_{11}(t_k) - 2\tilde{q}_1(t_k) \tilde{q}_2(t_k) \tilde{V}_{12}(t_k)}{2|\tilde{\mathbf{V}}|} \right). \quad (94)$$

Because the determinant  $|\tilde{\mathbf{V}}|$  is independent of  $\delta\phi$ , the log-likelihood is, up to multiplicative and additive constants that do not depend on  $\delta\phi$ :

$$\ell = - \sum_k \tilde{q}_1(t_k)^2 \tilde{V}_{22}(t_k) + \tilde{q}_1(t_k)^2 \tilde{V}_{22}(t_k) - 2\tilde{q}_1(t_k)\tilde{q}_2(t_k)\tilde{V}_{12}(t_k) \quad (95)$$

We maximize  $\ell$  with respect to  $\delta\phi_n := \delta\phi(t_n)$  for a given  $n \in \mathbb{Z}$ . This is attained when  $\partial\ell/\partial(\delta\phi_n) = 0$ . From eq. (92), we have

$$\frac{\partial\tilde{V}_{11}(t_k)}{\partial(\delta\phi_n)} = \frac{\Delta\Omega(V_+ - V_-)}{2\pi} \cos(\delta\phi_n) \delta_{k,n} = -\frac{\partial\tilde{V}_{22}(t_k)}{\partial(\delta\phi_n)} \quad (96)$$

$$\frac{\partial\tilde{V}_{12}(t_k)}{\partial(\delta\phi_n)} = \frac{\Delta\Omega(V_+ - V_-)}{2\pi} \sin(\delta\phi_n) \delta_{k,n} \quad (97)$$

Thus

$$\frac{\partial\ell}{\partial(\delta\phi_n)} = -\frac{\Delta\Omega(V_+ - V_-)}{2\pi} \left[ (-\tilde{q}_1(t_n)^2 + \tilde{q}_2(t_n)^2) \cos(\delta\phi_n) - 2\tilde{q}_1(t_n)\tilde{q}_2(t_n) \sin(\delta\phi_n) \right] = 0 \quad (98)$$

At lowest order in  $\delta\phi_n$ , we have  $\langle \tilde{q}_1(t_n)\tilde{q}_2(t_n) \rangle = \frac{(V_- - V_+)\Delta\Omega}{2\pi}$  from which we construct the maximum likelihood estimator that solves the previous equation on average:

$$\delta\phi^{\text{MLE}}(t_n) = \pi \frac{\tilde{q}_1(t_n)^2 - \tilde{q}_2(t_n)^2}{\Delta\Omega(V_+ - V_-)} \quad (99)$$

which corresponds to our proposed estimator eq. (75) under the approximation that  $H^2[\Omega] \simeq \Delta\Omega/\pi$ , which is valid in our range of frequencies  $\Omega \ll \Delta\Omega$ .

#### IV. CONTROL OF THE SQUEEZED FIELDS USING COHERENT LOCKING FIELDS

To stabilize the experiment, we require several control loops, which either actively control phases on the squeezers themselves, or the different phases intervening in the MZI transfer function eq. (31), to keep them at the setpoint values of eq. (33) for optimal estimation. There are two control loops (one per squeezer) to stabilize the relative phases between the pump fields ( $\psi_c$  for the CSQZ and  $\psi_b$  for the BOPA with convention  $\psi = 0$  for antisqueezing on the  $q$  quadrature) and the input CLF fields ( $\phi_{\text{CLF},c}$  and  $\phi_{\text{CLF},b}$ ). They are explained in section IV B.

There are four active control loops to be considered in locking the angles present in the MZI transfer function eq. (31):

- The Squeezing Angle Control (SAC), section IV C, stabilizes the relative angle of the input squeezed fields to  $\theta_s$ . This is a double-lock scheme that uses an auxiliary local oscillator (of phase  $\phi_{\text{LO},\text{sac}}$ ) to amplify the optical beatnotes;
- The MZI's differential phase loop, section IV D, stabilizes the differential path length ( $\phi_1 - \phi_2$ ) of the two arms of the MZI to keep it on gray fringe;
- The CLF-LO loop on the first (resp. second) homodyne detector, section IV E, stabilizes the relative phase between the incident squeezed field and the local oscillator of the homodyne detector  $\theta_1 + \frac{\phi_c}{2}$  (resp.  $\theta_2 + \frac{\phi_c}{2}$ )

At the output of the MZI, there are two sets of CLF fields copropagating with the squeezed field itself, one pair of sidebands per squeezer. The two CLF-LO locks of the homodynes both only use the CLF from the CSQZ. The CLF of the BOPA is only used for the Pump-CLF loop of the BOPA and the SAC loop.

#### A. Notations

In this section, we find convenient to work using the ladder vector basis  $\mathbf{a}[\Omega]$ , so unless otherwise specified, all matrices act on this basis.

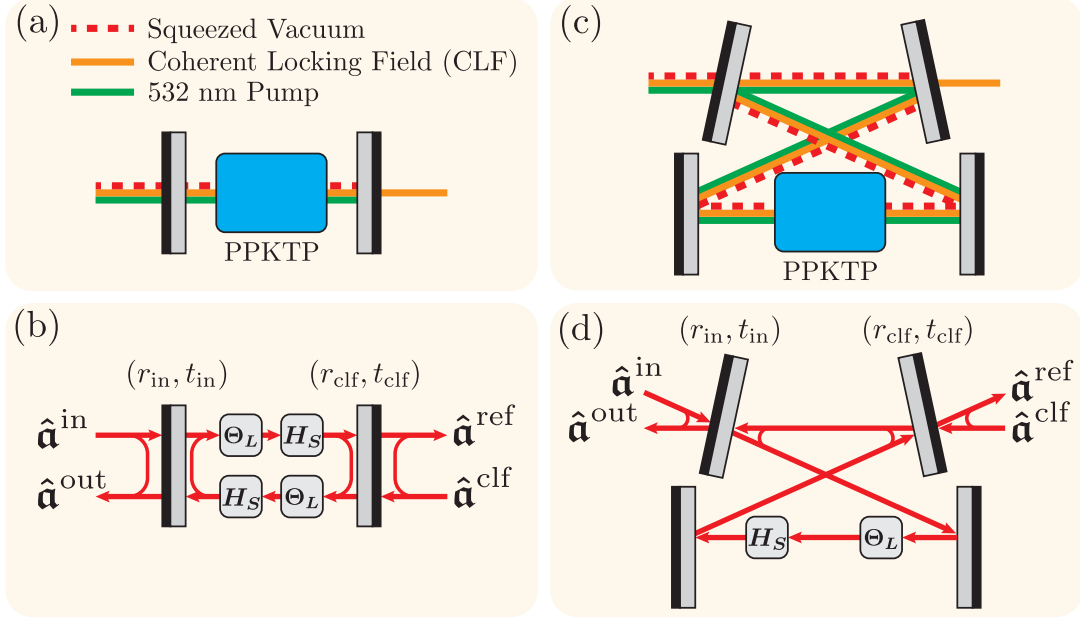

FIG. 2. OPA models. (a) and (c) show schematic representations of linear and bowtie OPAs respectively. (b) and (d) represent mathematical models of these OPAs, where  $\Theta_L$  represents the free propagation matrix while  $H_S$  represents the single pass squeezer matrix. Both types of OPA consist of a relatively low reflectivity input mirror with amplitude reflectivity  $r_{\text{in}}$  and transmissivity  $t_{\text{in}}$  and a highly, but not perfectly, reflective CLF mirror with amplitude reflectivity  $r_{\text{clf}}$  and transmissivity  $t_{\text{clf}}$

A single pass through a squeezer crystal is represented by  $H_S$ :

$$H_S = \begin{bmatrix} \cosh z & e^{2i\psi_p} \sinh z \\ e^{-2i\psi_p} \sinh z & \cosh z \end{bmatrix} \quad (100)$$

where  $z$  is the squeezing amplitude of a single pass and  $\psi_p$  is the phase of the pump field ( $\psi_p = \psi_c$  for CSQZ and  $= \psi_b$  for BOPA).

The cavity length propagation matrix is  $\Theta_L$ :

$$\Theta_L = e^{i\Omega\tau} \begin{bmatrix} e^{-i\Delta} & 0 \\ 0 & e^{i\Delta} \end{bmatrix} \quad (101)$$

with  $L$  the half-length of the linear cavity, or the full length of the bowtie cavity, and for sideband frequency  $\Omega$ ,

$$\Omega\tau = \frac{\Omega L}{c} = \frac{\Omega}{2f_{\text{FSR}}} \quad \text{and} \quad \Delta = \frac{\omega_0 L}{c} = \frac{\omega_0}{2f_{\text{FSR}}}. \quad (102)$$

In the following, we assume that the cavity is locked on resonance so  $\Delta = 0$ .

The relevant transfer matrices for the linear cavity (CSQZ, fig. 2 (a) and (b)) [5]:

$$\begin{aligned} \bar{H}^{\text{out},\text{in}}[\Omega] &= \left[ \mathbf{1} - r_{\text{in}} r_{\text{clf}} (H_S \Theta_L)^2 \right]^{-1} \times \left[ r_{\text{in}} - r_{\text{clf}} (H_S \Theta_L)^2 \right] \\ \bar{H}^{\text{out},\text{clf}}[\Omega] &= t_{\text{in}} t_{\text{clf}} \left[ \mathbf{1} - r_{\text{in}} r_{\text{clf}} (H_S \Theta_L)^2 \right]^{-1} H_S \Theta_L. \end{aligned} \quad (103)$$

And for the bowtie cavity (BOPA, fig. 2 (c) and (d)):

$$\begin{aligned} \bar{H}^{\text{out},\text{in}}[\Omega] &= r_{\text{in}} - r_{\text{clf}} t_{\text{in}}^2 [1 - r_{\text{in}} r_{\text{clf}} H_S \Theta_L]^{-1} H_S \Theta_L \\ \bar{H}^{\text{out},\text{clf}}[\Omega] &= t_{\text{in}} t_{\text{clf}} [1 - r_{\text{in}} r_{\text{clf}} H_S \Theta_L]^{-1}. \end{aligned} \quad (104)$$

Concretely, this means that for an incoming monochromatic CLF at frequency  $\Omega_{\text{CLF}}$  detuned from the carrier, the (classical) field into either OPA is of the form

$$E^{\text{CLF},\text{in}}(t) = 2E_0 |\bar{a}_{\text{CLF}}| \cos[(\omega_0 + \Omega_{\text{CLF}})t + \phi_{\text{CLF}}] \quad (105)$$

where  $E_0$  is some normalization constant of the electric field,  $\bar{a}_{\text{CLF}} = |\bar{a}_{\text{CLF}}|e^{-i\phi_{\text{CLF}}}$  is the complex amplitude of the field in photon flux units. The transmitted field is

$$E^{\text{tr}}(t) = 2E_0 \left\{ |\bar{a}_+^{\text{tr}}| \cos[(\omega_\ell + \Omega_{\text{CLF}})t + \phi_+^{\text{tr}}] + |\bar{a}_-^{\text{tr}}| \cos[(\omega_\ell - \Omega_{\text{CLF}})t + \phi_-^{\text{tr}}] \right\}, \quad (106)$$

where

$$|\bar{a}_+^{\text{tr}}| = |\bar{a}_{\text{CLF}}| |\bar{H}_{11}^{\text{tr}}[\Omega_{\text{CLF}}]|, \quad |\bar{a}_-^{\text{tr}}| = |\bar{a}_{\text{CLF}}| |\bar{H}_{12}^{\text{tr}}[-\Omega_{\text{CLF}}]| \quad (107)$$

$$\phi_+^{\text{tr}} = \phi_{\text{CLF}} - \arg(\bar{H}_{11}^{\text{tr}}[\Omega_{\text{CLF}}]), \quad \phi_-^{\text{tr}} = -\phi_{\text{CLF}} - \arg(\bar{H}_{12}^{\text{tr}}[-\Omega_{\text{CLF}}]), \quad (108)$$

and the reflected field is

$$E^{\text{ref}}(t) = 2E_0 \left\{ |\bar{a}_+^{\text{ref}}| \cos[(\omega_\ell + \Omega_{\text{CLF}})t + \phi_+^{\text{ref}}] + |\bar{a}_-^{\text{ref}}| \cos[(\omega_\ell - \Omega_{\text{CLF}})t + \phi_-^{\text{ref}}] \right\}, \quad (109)$$

where

$$|\bar{a}_+^{\text{ref}}| = |\bar{a}_{\text{CLF}}| |\bar{H}_{11}^{\text{ref}}[\Omega_{\text{CLF}}]|, \quad |\bar{a}_-^{\text{ref}}| = |\bar{a}_{\text{CLF}}| |\bar{H}_{12}^{\text{ref}}[-\Omega_{\text{CLF}}]| \quad (110)$$

$$\phi_+^{\text{ref}} = \phi_{\text{CLF}} - \arg(\bar{H}_{11}^{\text{ref}}[\Omega_{\text{CLF}}]), \quad \phi_-^{\text{ref}} = -\phi_{\text{CLF}} - \arg(\bar{H}_{12}^{\text{ref}}[-\Omega_{\text{CLF}}]). \quad (111)$$

## B. The CLF-Pump loops

The CLF-Pump loop locks the phases of the two sidebands at  $\pm\Omega_{\text{CLF}}$  on reflection of the OPA. Indirectly, this locks the CLF input phase  $\phi_{\text{CLF}}$  with the squeezing angle  $\psi$ , since the information on the latter is contained in the phases of the fields in reflection  $\phi_\pm^{\text{ref}}$ . Since the principle of this loop is identical for either CSQZ or BOPA, here  $\psi$  (and  $\phi_{\text{CLF}}$ ) can be  $\psi_c$  ( $\phi_{\text{CLF},c}$ ) or  $\psi_b$  ( $\phi_{\text{CLF},b}$ ).

More precisely, one looks at the power at  $2\Omega_{\text{CLF}}$ ,  $P_{2\Omega_{\text{CLF}}}(t)$  in the reflected field (eq. (109)) from the cavity:

$$P_{2\Omega_{\text{CLF}}}(t) := E^{\text{ref}}(t)^2|_{2\Omega_{\text{CLF}}} = 4E_0^2 |\bar{a}_+^{\text{ref}}| |\bar{a}_-^{\text{ref}}| \cos(2\Omega t + \phi_+^{\text{ref}} - \phi_-^{\text{ref}}) \quad (112)$$

Demodulating this at  $2\Omega_{\text{CLF}}$  with some demodulation angle allows to establish a lock between  $\phi_+^{\text{ref}}$  and  $\phi_-^{\text{ref}}$ :

$$\phi_+^{\text{ref}} = \phi_-^{\text{ref}} + \text{const.} \quad (113)$$

Since both can be expressed as a function of  $\psi$  and  $\phi_{\text{CLF}}$ , we have effectively locked them together. In other words, we see that the loop allows to arbitrarily set the phase  $\phi_{\text{Lock}}$ :

$$\phi_{\text{Lock}} := \phi_+^{\text{ref}} - \phi_-^{\text{ref}} = 2\phi_{\text{CLF}} - \arg(\bar{H}_{11}^{\text{ref}}[\Omega_{\text{CLF}}]) + \arg(\bar{H}_{12}^{\text{ref}}[-\Omega_{\text{CLF}}]) \quad (114)$$

Absorbing constants into  $\phi_{\text{Lock}}$  (which amounts to defining  $\phi_{\text{Lock}}$  up to some arbitrary reference phase) leads to the simple relation

$$\phi_{\text{Lock}} = 2\phi_{\text{CLF}} + 2\psi \quad (115)$$

where experimentally, we can choose the lock setpoint  $\phi_{\text{Lock}}$ . This means that in the frame of the CLF, we are free to set the pump phase. In the following, we choose without loss of generality  $\psi_c = 0$  in the frame of the CSQZ CLF, but  $\psi_b \neq 0$  since the BOPA CLF's frame is not a priori phase-locked to that of the CSQZ CLF. This is the purpose of the squeezing angle control feedback loop discussed in the next section.

## C. The Squeezing Angle Control loop

The SAC is composed of a succession of CLF-LO loops. It reproduces the scheme introduced in [6] to achieve stable control of the relative phase angle between two squeezed fields. Each CLF-LO loop consists locks the phase of the beatnote at  $\Omega_{\text{CLF}}$  between the transmitted field from the OPA, picked off in the MZI, with the LO field on a fiber-coupled PD. This is preferred over the direct lock on the beatnote of the two CLF fields because of the very low amplitude of the latter as compared to an effective amplification thanks to the bright LO field. We denote  $\phi_{\text{LO},\text{sac}}$  the phase of this LO field, which will have to be locked on either CLF phases.

The relative squeeze angle control consists in the following steps:

- Lock the relative phase of  $\phi_{\text{LO,sac}}$  and  $\phi_{\text{CLF,c}}$ , defined as  $\phi'_{\text{Lock,c}}$  with feedback on  $\phi_{\text{LO,sac}}$ .
- Lock the relative phase of  $\phi_{\text{LO,sac}}$  and  $\phi_{\text{CLF,b}}$ , defined as  $\phi'_{\text{Lock,b}}$  with feedback on  $\psi_b$ .

For simplicity, we write the transmitted transfer function of the CSQZ as  $H^c$  and that of the BOPA as  $H^b$ . Each lock between a CLF field and its LO corresponds to setting the angles

$$\phi'_{\text{Lock,c}} = \phi_{\text{CLF,c}} + \arg \left( \bar{H}_{11}^c [\Omega_{\text{CLF,c}}]^* e^{-i\phi^{\text{LO,sac}}} + \bar{H}_{12}^c [-\Omega_{\text{CLF,c}}] e^{i(\phi^{\text{LO,sac}} + \psi_c)} e^{i\psi_c} \right) \quad (116)$$

$$\phi'_{\text{Lock,b}} = \phi_{\text{CLF,b}} + \arg \left( \bar{H}_{11}^b [\Omega_{\text{CLF,b}}]^* e^{-i\phi^{\text{LO,sac}}} + \bar{H}_{12}^b [-\Omega_{\text{CLF,b}}] e^{i(\phi^{\text{LO,sac}} + \psi_b)} e^{i\psi_b} \right) \quad (117)$$

(see derivation in section IV E). To map the physical phase to the demodulation phase, we want to find the transformation between  $\phi'_{\text{Lock,b}}$  and  $\psi_b$ . We can write two relevant maps, with different offset phases:  $\phi_{\text{LO,sac}} = f(\phi'_{\text{Lock,c}})$  and  $\psi_b = g(\phi_{\text{LO,sac}})$ . By inverting this map, it is possible to set the relative squeezing angle  $\theta_s = \psi_b - \psi_c = \psi_b$  to the setpoint in eq. (33).

#### D. MZI differential arm length lock

This lock is obtained by picking off  $\kappa = 1\%$  of each of the two outputs of the MZI and sending them to a pair of balanced photodiodes. Denoting the power of the fields the input of the MZI as  $P_1^{\text{in}}(t)$  and  $P_2^{\text{in}}(t)$ , the outputs are

$$P_1^{\text{out}}(t) = \kappa \left[ \cos^2 \left( \frac{\phi_d}{2} \right) P_1^{\text{in}}(t) + \sin^2 \left( \frac{\phi_d}{2} \right) P_2^{\text{in}}(t) \right] \quad \text{and} \quad P_2^{\text{out}}(t) = \kappa \left[ \sin^2 \left( \frac{\phi_d}{2} \right) P_1^{\text{in}}(t) + \cos^2 \left( \frac{\phi_d}{2} \right) P_2^{\text{in}}(t) \right] \quad (118)$$

Thus the differential output of the balanced photodetector is

$$P_1^{\text{out}}(t) - P_2^{\text{out}}(t) = \kappa \frac{\cos(\phi_d)}{2} (P_1^{\text{in}}(t) - P_2^{\text{in}}(t)) \quad (119)$$

Since in our experiment,  $P_1^{\text{out}}(t) \neq P_2^{\text{out}}(t)$ , this expression is null at all times only if  $\phi_d = \pi/2$  (up to integer multiple of  $\pi$ ). This provides the correct error signal to lock on the required gray fringe of eq. (33).

#### E. CLF-LO loop for Homodyne Detectors

As stated previously, for the CLF-LO loops on both homodynes we only use the beatnotes at the frequency of the CSQZ's CLF. For the calculations it thus suffices to only propagate this CLF through the MZI interferometer. The classical field with CLF component transmitted out of the CSQZ is (eq. (106))

$$E^{\text{tr}}(t) = 2E_0 \left\{ |\bar{a}_+^{\text{tr}}| \cos[(\omega_\ell + \Omega_{\text{CLF}})t + \phi_+^{\text{tr}}] + |\bar{a}_-^{\text{tr}}| \cos[(\omega_\ell - \Omega_{\text{CLF}})t + \phi_-^{\text{tr}}] \right\} \quad (120)$$

The MZI locked on a gray fringe simply imparts a common phase delay to the previous expression, which corresponds to both the outputs of the MZI up to a multiplicative factor of  $1/\sqrt{2}$  which can be absorbed in  $E_0$ , and an overall phase  $\phi_c/2$  which can be absorbed in  $\phi_\pm^{\text{tr}}$ . In the following, we consider either homodyne detector.

The local oscillator impinging on the homodyne detector has a field of the form

$$E^{\text{LO}}(t) = 2E_0 |\bar{a}^{\text{LO}}| \cos[\omega_\ell t + \phi^{\text{LO}}], \quad (121)$$

so the beatnote  $P_{\Omega_{\text{CLF}}}(t)$  between the LO and the CLF at  $\Omega_{\text{CLF}}$  is

$$P_{\Omega_{\text{CLF}}}(t) = [E^{\text{tr}}(t) + E^{\text{LO}}(t)]^2|_{\Omega_{\text{CLF}}} = 2E^{\text{tr}}(t)E^{\text{LO}}(t)|_{\Omega_{\text{CLF}}} \quad (122)$$

$$= 8E_0^2 |\bar{a}^{\text{LO}}| |\bar{a}_{\text{CLF}}| \left[ |\bar{H}_{11}^{\text{tr}}[\Omega_{\text{CLF}}]| \cos(\Omega_{\text{CLF}}t + \phi_+^{\text{tr}} - \phi^{\text{LO}}) + |\bar{H}_{12}^{\text{tr}}[-\Omega_{\text{CLF}}]| \cos(\Omega_{\text{CLF}}t + \phi_-^{\text{tr}} - \phi^{\text{LO}}) \right] \quad (123)$$

$$= 2|P_{\Omega_{\text{CLF}}}| \cos(\Omega_{\text{CLF}}t + \theta_{\text{CLF-LO}}), \quad (124)$$

where

$$|P_{\Omega_{\text{CLF}}}| = 8E_0^2 |\bar{a}^{\text{LO}}| |\bar{a}_{\text{CLF}}| \left| \bar{H}_{11}^{\text{tr}}[\Omega_{\text{CLF}}]^* e^{-i\phi^{\text{LO}}} + \bar{H}_{12}^{\text{tr}}[-\Omega_{\text{CLF}}] e^{i\phi^{\text{LO}}} \right| \quad (125)$$



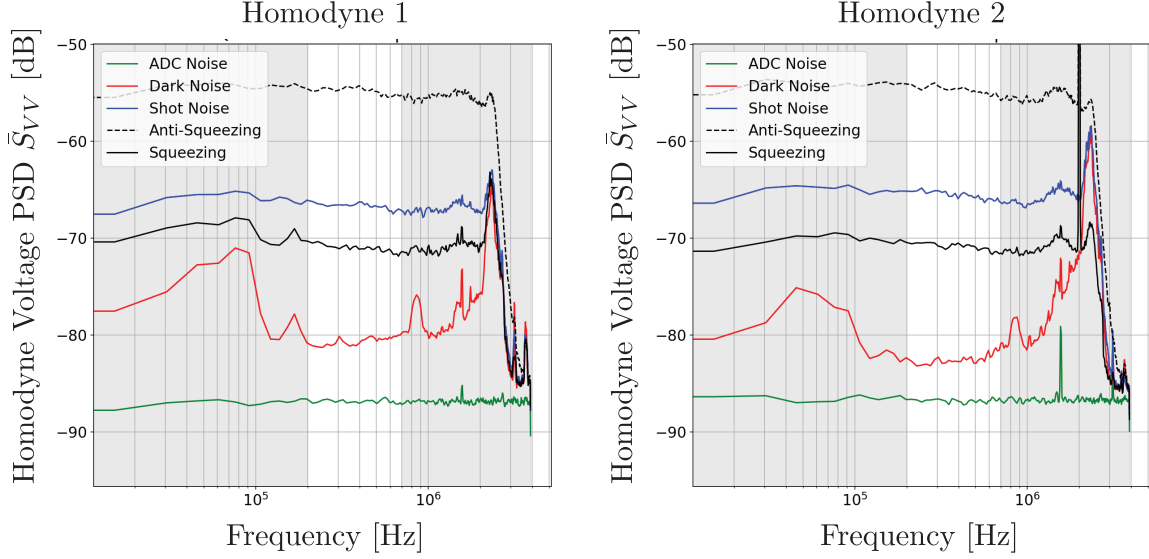

FIG. 3. Homodyne noise measurements for the two homodyne detectors used in the squeezed light interferometer experiments. The region between 200 kHz and 700 kHz, used to determine the experiment's squeezing levels and for interferometer phase estimation is highlighted.

and

$$\theta_{\text{CLF-LO}} = \phi_{\text{CLF}} + \arg \left( \bar{H}_{11}^{\text{tr}}[\Omega_{\text{CLF}}]^* e^{-i\phi^{\text{LO}}} + \bar{H}_{12}^{\text{tr}}[-\Omega_{\text{CLF}}] e^{i\phi^{\text{LO}}} \right). \quad (126)$$

Recall that closing the loop amounts to fixing the argument  $\theta_{\text{CLF-LO}}$  to some setpoint  $\phi'_{\text{Lock}}$  (demodulation phase). Because  $\phi_{\text{CLF}}$  is already fixed by the CLF-pump loop eq. (115), we obtain a one-to-one map between the demodulation angle  $\phi'_{\text{Lock}}$  and the homodyne readout angle  $\phi^{\text{LO}} = \theta_{1,2} + \phi_c/2$  using the notations of the setpoint requirement in eq. (33).

## V. EXPERIMENTAL CALIBRATION MEASUREMENTS

### A. Homodyne Detectors and Squeezing Measurements

We measure squeezing using custom-built homodyne detectors. Figure 3 shows shot noise, dark noise, squeezing, and anti-squeezing from each of the two homodynes used in the experiment. To measure these noise levels, we passed the output voltage of the homodyne detectors through a 2 MHz anti-aliasing filter and digitized the resulting voltage with a Picoscope 4227 with a 7 MHz sampling frequency (3.5 MHz Nyquist frequency). We then used the Welch method to estimate the PSDs from the digitized homodyne signals. The roll-off from the anti-aliasing filter is evident in these measurements.

We see that between 200 kHz and 700 kHz, shot noise exceeds dark noise by 13.8 dB on average on homodyne 1, and 16.8 dB on homodyne 2, corresponding to effective losses of 4.0% and 2.0%, respectively. The ADC noise characterizes the noise floor of the Picoscope used for data acquisition. This data was taken with its inputs terminated with 50 ohm resistors and is the only dataset acquired with no 2 MHz anti-aliasing filter. Dark noise was measured from the homodynes, through the anti-aliasing filter, with the local oscillator beam turned off and the path from the OPAs to the homodyne blocked with a beam stop. Shot noise was measured with the local oscillator beam turned on, at the power level used in all successive experiments, and the path from the OPAs to the homodyne detectors blocked with beam stops. Squeezing (anti-squeezing) was measured by scanning the homodyne demodulation angle and identifying the measurement with the most shot noise suppression (amplification).

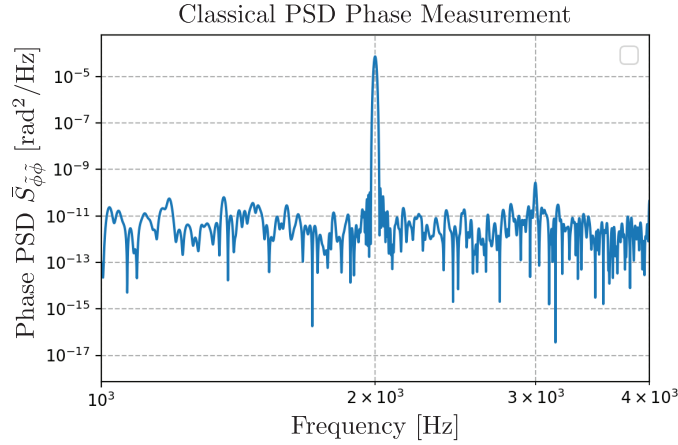

FIG. 4. The estimated interferometer differential phase power spectral density measured using a laser beam. The modulation tone at 2 kHz is clearly visible above the noise floor.

### B. Classical Calibration of Phase Modulation Tone

To validate that our estimator is unbiased and that it faithfully reconstructs an injected phase modulation tone, we measured the interferometer phase classically, using well-established interferometric methods. To generate a classical beam, we sent 10s of mW of laser power into the CLF port of one of the two OPAs and dither locked the OPA to this laser beam. The beam transmitted through the OPA then has the same mode shape as the squeezed beam would and was sent through the interferometer. The other OPA was turned off during this measurement. We then drove the interferometer's differential phase with a large, low-frequency modulation tone such that the interferometer swept through several fringes and recorded the peak-to-peak voltage,  $V_{pp}^{\max}$ , measured with our high-gain differential receiver and digitized with a Red Pitaya FPGA.

We then used turned off the low frequency modulation tone and locked the interferometer mid-fringe using the classical field. We locked the interferometer with the same unity gain frequency of 1 kHz and same feedback loop shape as in the quantum measurement discussed in the main text. We injected the same 2 kHz modulation tone as in the quantum measurement and recorded the resulting voltage PSD using the same differential receiver and Red Pitaya FPGA.

We used Welch's method to convert the measured voltage signal with the modulation tone to a PSD,  $\bar{S}_{VV}[\Omega]$ . For an interferometer locked mid-fringe, the phase PSD,  $\bar{S}_{\phi\phi}$ , is related to this voltage PSD through  $V_{pp}^{\max}$  via

$$\bar{S}_{\phi\phi}[\Omega] = \frac{4\bar{S}_{VV}[\Omega]}{(V_{pp}^{\max})^2}. \quad (127)$$

The resulting phase PSD is shown in fig. 4. We integrate this phase PSD in a narrow band around 2 kHz to extract the RMS phase modulation, which we find to be 75.3 mrad.

### C. Estimator Linearity

To estimate the interferometer's differential phase in our squeezed light interferometer, we use a linearized MLE as discussed above and in the main text. If the interferometer's differential phase modulation is too large, we expect this assumption to break down and our estimator to become biased such that the spectral QCRB no longer applies. To verify that our estimated phase is linear in the interferometer's differential phase, we take a series of sequential measurements with the modulation amplitude reduced by 50% in each measurement. We find that the estimated phase RMS is linear and agrees well with the classical measurements, denoted by the dashed gray line in fig. 5. This line is computed using the classical measurement and the fact that the modulation amplitude is decreased by 50% at each successive data point, and is not a curve fit.

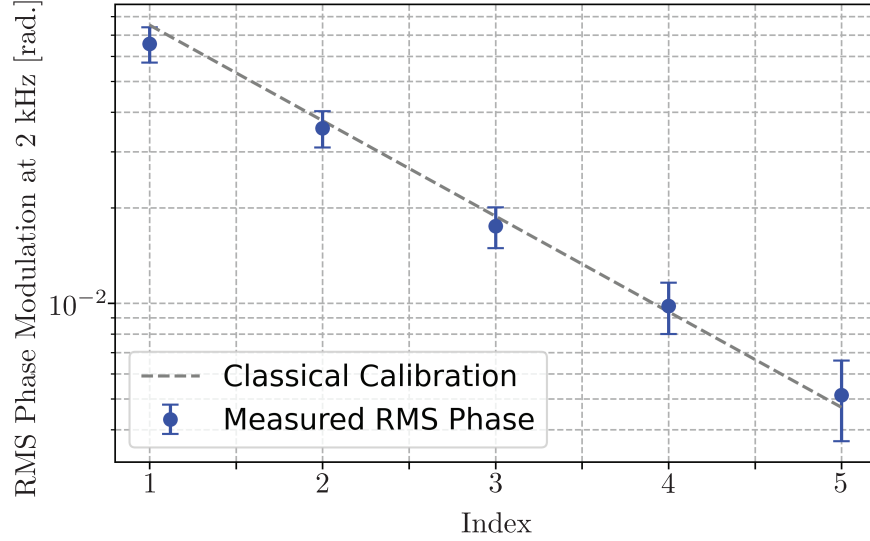

FIG. 5. Estimated RMS phase vs index for the squeezed light interferometer and a classical measurement. At each index, the modulation amplitude is decreased 50%. The error bars are 2-sigma error bars. The classical measurement described in section VB determines the value of the classical (dashed gray) curve for index 1 and the slope is given by 50% decrease in modulation amplitude at each successive index.

## VI. SYMMETRY AND STABILITY CRITERIA FOR ACCEPTING DATA POINTS

As discussed in Methods, we adopt the following criteria to accept a data point. Otherwise the data point is vetoed and is not considered in the rest of our analysis.

1. The estimator is sufficiently un-biased: The measured RMS phase modulation at 2 kHz is within 30% of the value obtained through a separate, classical measurement.
2. Demodulation phase stability: The phase estimation PSD noise floor obtained after returning to the optimal demodulation phases determined by the SNR heatmap (see main text fig. 2(f)) is within 30% of the value measured while taking the heatmap.
3. Photon number stability: The photon flux through the interferometer did not drift by more than 30% over the course of the measurement.
4. Low loss: The experimentally measured end-to-end loss is less than 30% before or after the phase PSD measurements and the mean measured loss before and after the phase PSD measurements is less than 35%.
5. Squeezer Symmetry: To ensure the squeezing levels are sufficiently symmetric after the OPA outputs are sent into the interferometer, we require that at the relative squeezing angle demodulation value corresponding to the lowest squeezing variance as the homodyne demodulation phase is scanned, the standard of deviation of homodyne variance divided by the maximum level of anti-squeezing is less than 0.15. This seems to be a reasonably heuristic to enforce the desired degree of symmetry.

To assess how these criteria affect our data, we plot all data points and their associated value for each relevant criteria in fig. 6.

We note that the loss is determined experimentally using the maximal levels of squeezing on either homodyne and the maximal levels of anti-squeezing on either homodyne. With  $V_{\text{sqz}}$  the variance corresponding to the maximal level of anti-squeezing and  $V_{\text{asqz}}$  the variance corresponding to the maximal level of squeezing in units such that shot noise corresponds to  $V_{\text{sqz}} = V_{\text{asqz}} = 1$ , the measured loss is

$$\eta^2 = \frac{V_{\text{sqz}}V_{\text{asqz}} - 1}{V_{\text{sqz}} + V_{\text{asqz}} - 2}. \quad (128)$$

We make several observations based on fig. 6. First, we accept slightly more than half of all attempts to make measurements with the experiment, so the underlying setup is reasonably stable. We observe that data points with

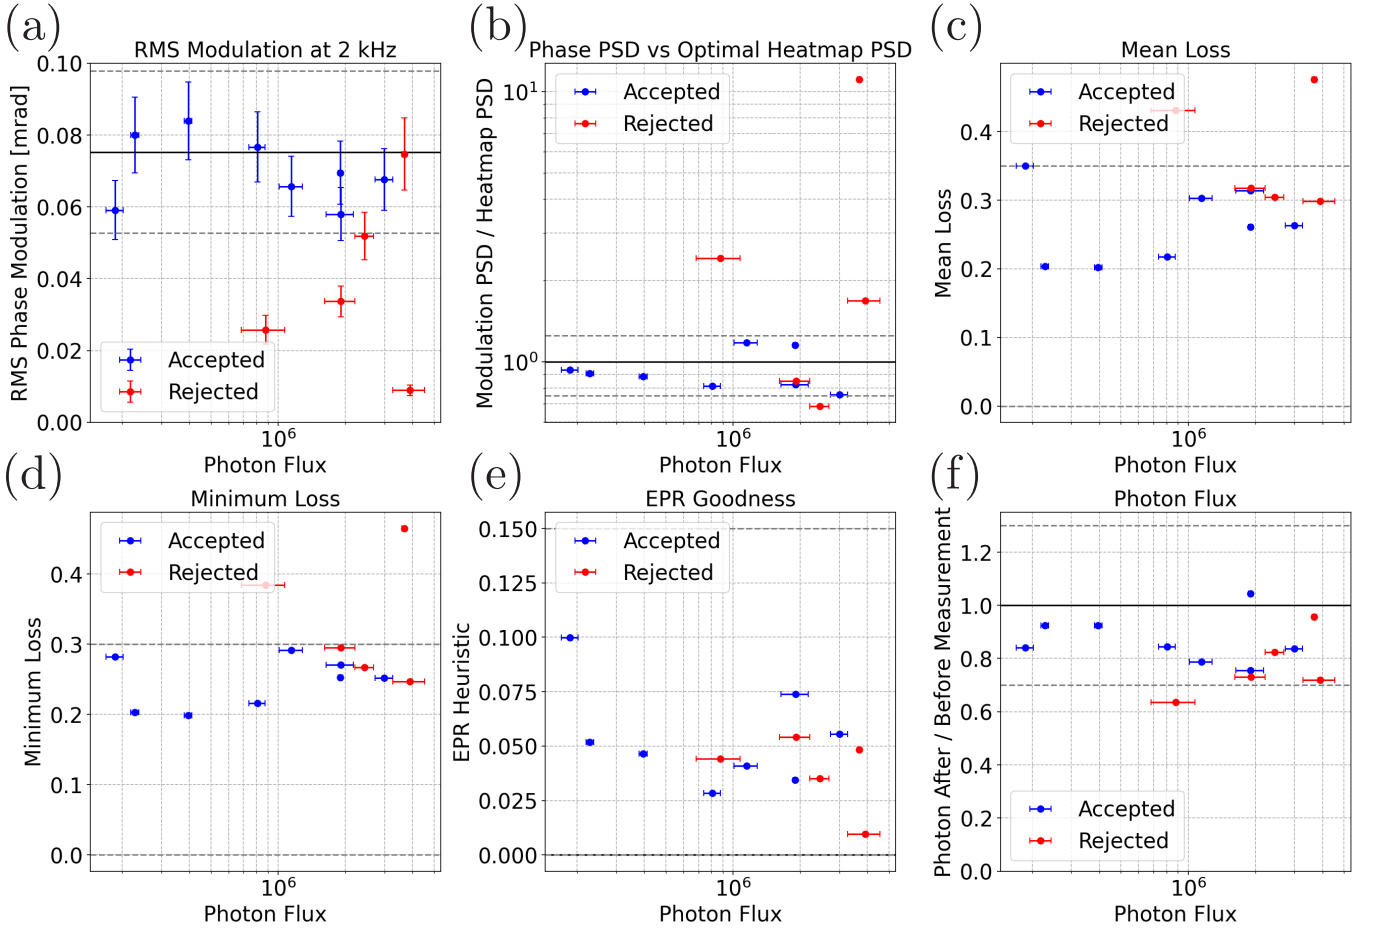

FIG. 6. A summary of all measured datasets compared with the criteria for accepting a data point. Accepted data points are shown in blue. Rejected, or vetoed, data points are shown in red. The region between the dashed gray lines contains data points that pass the specified criteria. All data points outside this region are rejected. Some data points inside this region may be rejected if they fail other criteria. All plots share the same x-axis. (a) The RMS modulation amplitude at 2 kHz. The y-axis error bars are two-sigma error bars from uncertainty in the PSD estimate. The solid black line is the classically measured value. (b) The phase PSD noise floor after returning to the optimal values of the demodulation phases divided by the phase PSD noise floor of the data point in the SNR heatmap with the highest SNR. The black horizontal line denotes the optimal value: the PSDs match exactly. (c) The mean measured loss from loss estimated before and after the phase PSD measurements. (d) The minimum loss from loss estimated before and after the phase PSD measurements. The black line denotes the optimum: the states are matched exactly and the value of the EPR heuristic vanishes. (e) The EPR heuristic. (f) Photon flux measured after the phase PSD measurements divided by photon flux measured before phase PSD measurements. The black line denotes the optimum: there is no drift.

higher photon fluxes are more likely to be rejected, indicating that the experiment is generally less stable with higher squeezing levels. We also observe that we did not need to include all of these criteria. For instance, the mean loss and RMS criteria (panels (a) and (c)) are sufficient to determine whether a data point is accepted or rejected by all six criteria plotted. However, we include all criteria as we believe the 11 measurement attempts we report here likely do not capture all of the ways in which the experiment can drift or change state over the course of taking data. We believe that future attempts to replicate or build off of these results may want to incorporate all of these criteria, as we have.

- 
- [1] K. J. Blow, R. Loudon, S. J. D. Phoenix, and T. J. Shepherd, Continuum fields in quantum optics, *Phys. Rev. A* **42**, 4102 (1990).
  - [2] S. L. Danilishin and F. Y. Khalili, Quantum measurement theory in gravitational-wave detectors, *Living Reviews in Relativity* **15**, 1 (2012).
  - [3] J. Ding, H. A. Loughlin, and V. Sudhir, Quantum linear time-translation-invariant systems: Conjugate symplectic structure, uncertainty bounds, and tomography, *arXiv:2410.09976* (2024).
  - [4] M. Tsang, H. M. Wiseman, and C. M. Caves, Fundamental quantum limit to waveform estimation, *Phys. Rev. Lett.* **106**, 090401 (2011).
  - [5] D. Ganapathy, V. Xu, W. Jia, C. Whittle, M. Tse, L. Barsotti, M. Evans, and L. McCuller, Probing squeezing for gravitational-wave detectors with an audio-band field, *Phys. Rev. D* **105**, 122005 (2022).
  - [6] T. Eberle, V. Händchen, and R. Schnabel, Stable control of 10 db two-mode squeezed vacuum states of light, *Opt. Express* **21**, 11546 (2013).
